# Supplementary material for: Transient Signal Propagation in Heterogeneous Networks under Various Inputs
Source: arXiv:2510.19481 source file (2026-11-17)
Supplement: Supplementary file 1 [file supp.tex]

\documentclass{article}
\usepackage{graphicx}
\usepackage{epstopdf}
\usepackage{subfigure}
\usepackage{amsmath}
\usepackage{geometry}
\usepackage{indentfirst}
\usepackage{graphicx}
\usepackage{multirow}
\usepackage{amsfonts}
\usepackage{verbatim}
\usepackage{appendix}
\usepackage{caption}
\usepackage{booktabs}
\usepackage{framed}
\usepackage{tikz}
\usepackage{makecell}
\usepackage{diagbox}
\usepackage{slashbox}
\usepackage{pifont}
\usepackage{cite}
\usepackage[greek,english]{babel}
\usepackage[OT2,OT1]{fontenc}
\usepackage{texnames}
\usepackage{mflogo}
\usepackage{amsmath} % for advanced math typesetting
\usepackage{amsfonts} % for mathematical fonts
\usepackage{amssymb} % for mathematical symbols
\usepackage{amsthm} % for defining theorem environments
\usepackage{hyperref}
\usepackage{cleveref}
\usepackage{autonum}

\pdfoptionpdfminorversion = 6
% Define theorem styles and environments

\theoremstyle{definition}

% Create a new command to conditionally !h equations only if they are referenced
\newcommand{\reflabeq}[2]{
  \ifcsname r@#2\endcsname
    \label{#2}
  \fi
  \begin{equation}
    #1
    \reflabeq{#2}
  \end{equation}
}

\setcounter{figure}{0}

\title{Supplementary Material}
\author{Xiaoge Bao, Wei P. Dai, Jan Nagler, Wei Lin}
%\date{}

%\renewcommand{\theequation}{S\arabic{equation}}
%\renewcommand{\thefigure}{S\arabic{figure}}
%\renewcommand{\thetable}{S\arabic{table}}

\begin{document}

\maketitle
\tableofcontents 

\clearpage

\section{Numerical accuracy test in NSDD system}
\label{supp:num}
\subsection{Constant input}
\label{supp:constant}
\begin{figure}[!ht]
\centerline{\includegraphics[scale=0.65]{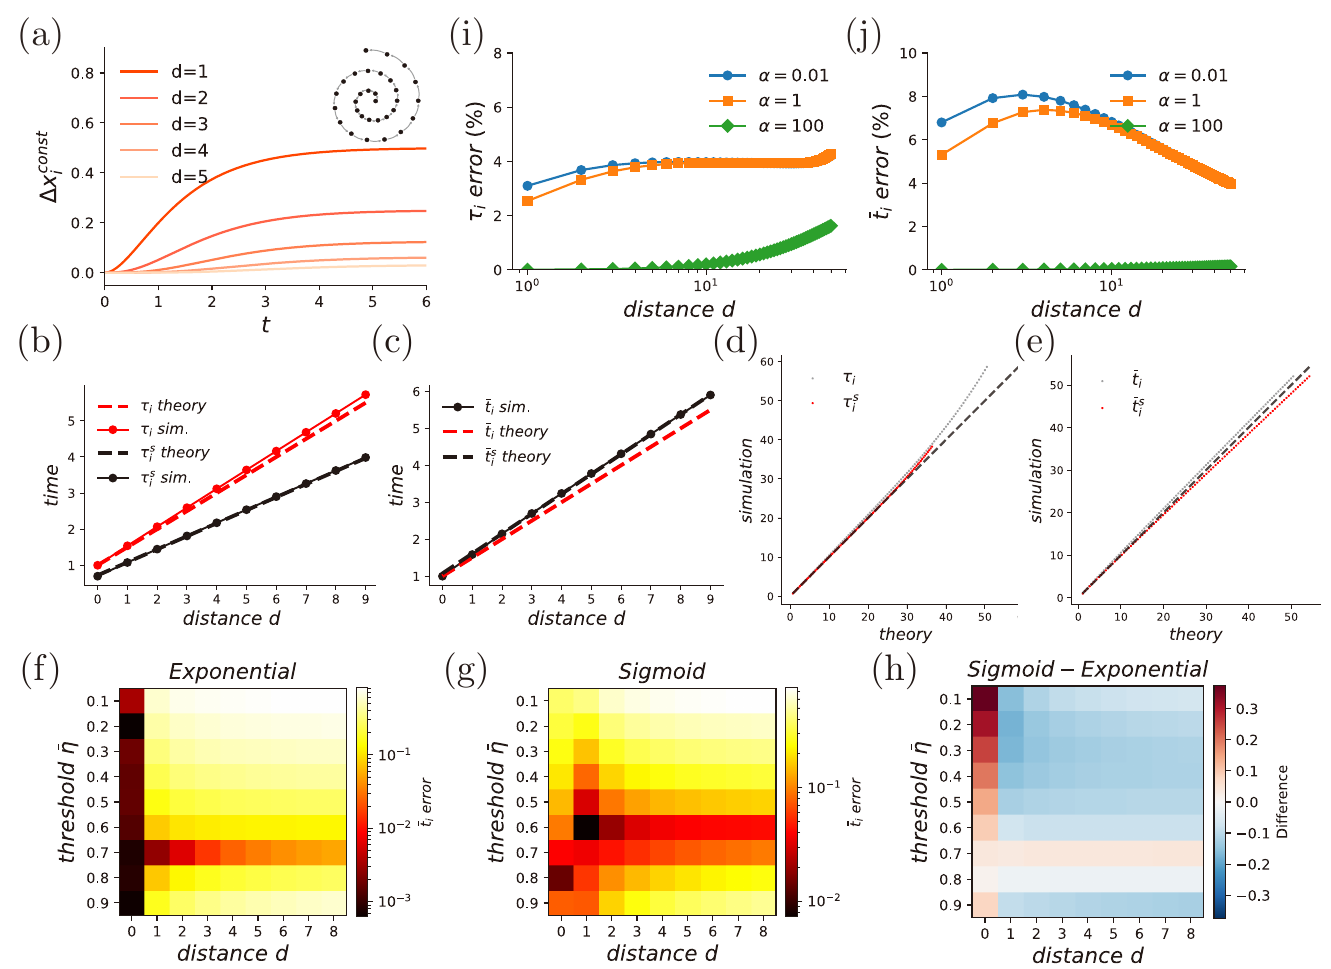}}
\caption{
Constant perturbation spreading through a directed chain of length $100$. All panels (a) to (h) use NSDD system parameters: topology matrix entries $\alpha = 1$ and self-decay parameter $\beta = 1$. The threshold $\bar{\eta} = 1-1/e$ is used in panels (c), (e), and (i). 
(a) Time courses for nodes at different shortest path lengths from input. 
(b) Simulated vs. theoretical time constants $\tau_i$ and $\tau_i^s$ (exponential and sigmoidal functions; dashed lines show simulations). 
(c) Simulated vs. theoretical relative propagation times $\bar{t}_i$ and $\bar{t}_i^s$ (exponential and sigmoidal; sigmoid shows better fit). 
(d) Simulated vs. theoretical time constants for exponential ($\tau_i$) and sigmoidal ($\tau_i^s$) functions (dotted lines indicate perfect match). 
(e) Simulated vs. theoretical relative propagation times for exponential ($\bar{t}_i$) and sigmoidal ($\bar{t}_i^s$) estimations. 
(f) Relative error in exponential fitting (minimum error near $\bar{\eta} \approx 0.7$). 
(g) Relative error in sigmoid fitting (minimum error near $\bar{\eta} \approx 0.6$). 
(h) Sigmoid vs. exponential relative error comparison (blue indicates superior sigmoid performance). 
(i) Time constant relative error vs. topological weights $\alpha$ (error decreases with larger $\alpha$, increases with distance). 
(j) Propagation time relative error vs. $\alpha$ (optimal distance for minimal error). 
Relative error for panels (f)-(j) is defined as $|\text{sim. } t - \text{thr. } t|/\text{sim. } t$.
}
\label{constant_chain}
\end{figure}

\begin{figure}[!ht]
\centerline{\includegraphics[scale=0.5]{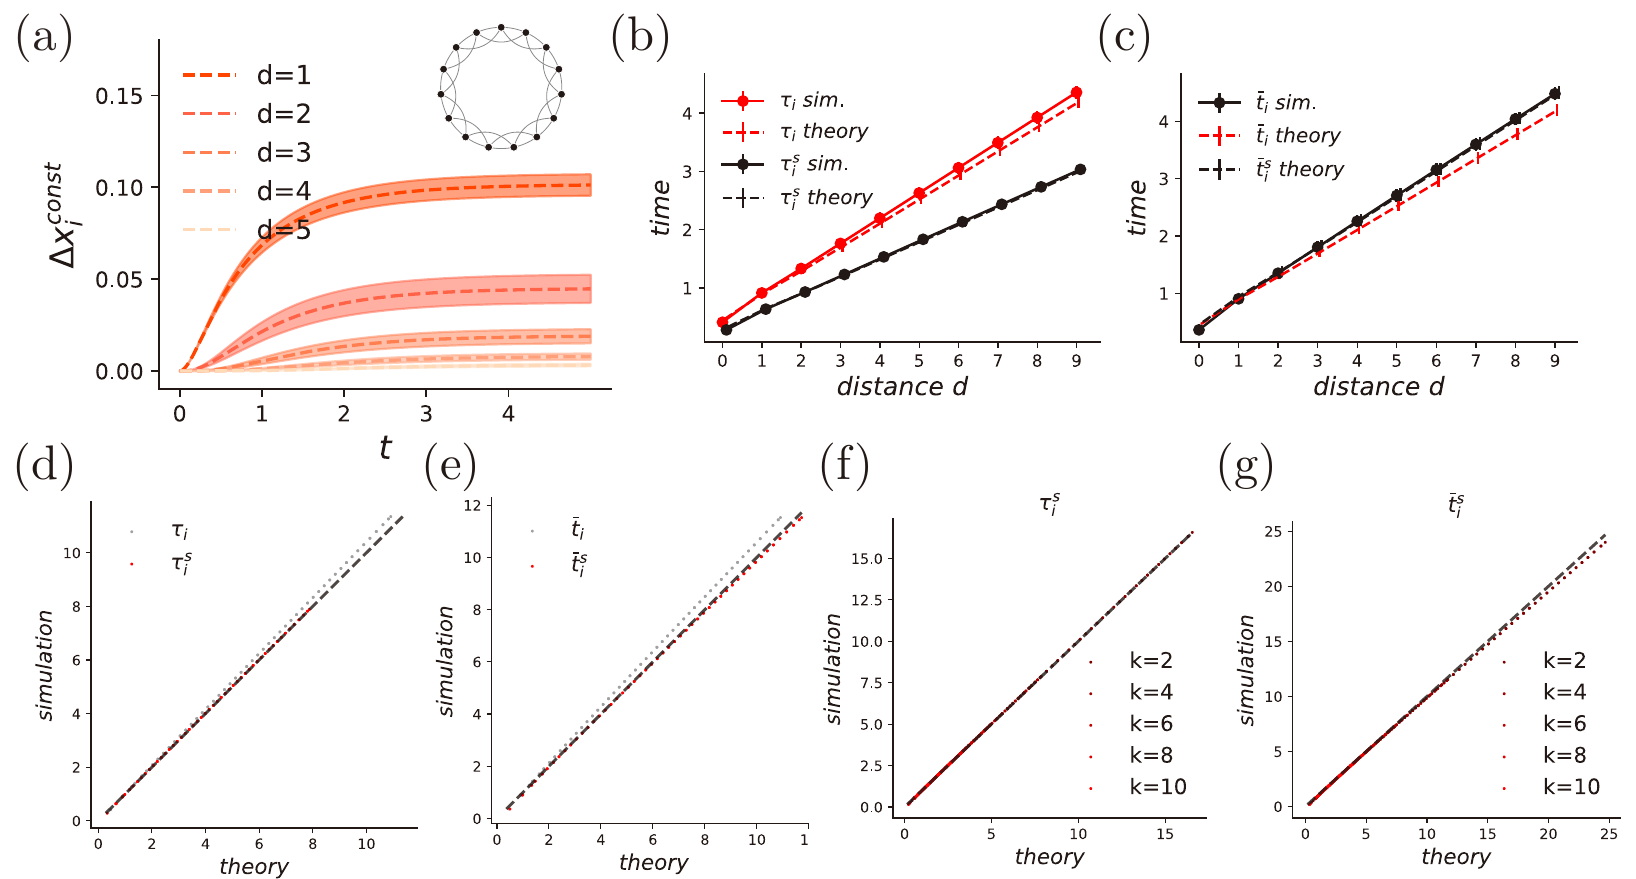}}
    \caption{
Constant perturbation spreads through a ring lattice of length $100$, with one input projecting to any node. The NSDD system uses topology matrix entries $\alpha = 1$ and self-decay parameter $\beta = 1$ for all panels (a) to (g), with the threshold $\bar{\eta} = 1-1/e$ in panels (c), (e), and (g). Nodes have degree $4$ in panels (a) to (e). (a) Time courses vs. shortest path lengths from input. (b) Simulated versus theoretical time constants $\tau_i$ and $\tau_i^s$ for exponential and sigmoidal functions (dashed lines: theoretical results). (c) Simulated versus theoretical relative propagation times $\bar{t}_i$ and $\bar{t}_i^s$ for exponential and sigmoidal functions (sigmoid shows better fit). (d) Simulated vs. theoretical time constants for exponential ($\tau_i$) and sigmoidal ($\tau_i^s$) functions (dotted lines: perfect matches). (e) Simulated versus theoretical relative propagation times for exponential ($\bar{t}_i$) and sigmoidal ($\bar{t}_i^s$) estimations. (f) Simulated vs. theoretical time constants for sigmoidal functions ($\tau_i^s$) across different node degrees. (g) Simulated versus theoretical relative propagation times for sigmoidal functions ($\bar{t}_i^s$) across different node degrees.
}
\label{constant_regular}
\end{figure}

\begin{figure}[!ht]
\centerline{\includegraphics[scale=0.78]{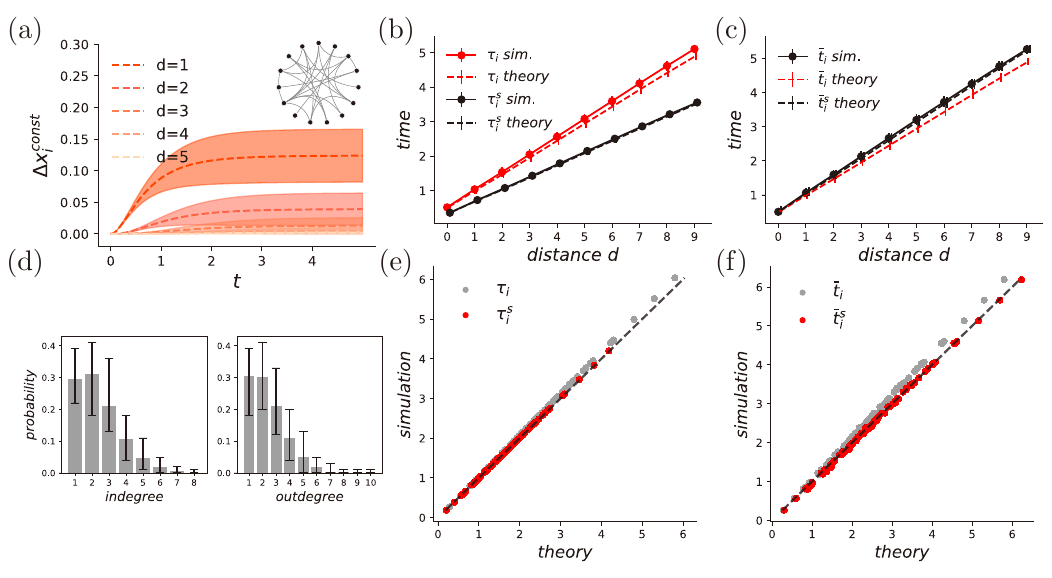}}
    \caption{
Constant perturbation spreading through an Erdős-Rényi random network ($N=100$ nodes) over $100$ simulation rounds, with one input projecting to random nodes. NSDD system parameters: $\alpha = 1$ (edge weights), $\beta = 1$ (self-decay), $\bar{\eta} = 1-1/e$ (decay threshold; c,f). (a) Time courses vs. shortest path lengths from input (shaded area: std. for same-path-length nodes). (b) Simulated vs. theoretical time constants $\tau_i$ and $\tau_i^s$ for exponential and sigmoidal functions (vertical lines: error ranges). (c) Simulated versus theoretical relative propagation times $\bar{t}_i$ and $\bar{t}_i^s$ for exponential and sigmoidal functions (sigmoid shows better fit; small errors). (d) In-degree and out-degree distributions. (e) Scatter plot: simulated versus theoretical time constants for exponential ($\tau_i$) and sigmoidal ($\tau_i^s$) functions across all rounds. (f) Scatter plot: simulated versus theoretical relative propagation times for exponential ($\bar{t}_i$) and sigmoidal ($\bar{t}_i^s$) functions across all rounds.
}
\label{constant_random}
\end{figure}

\begin{figure}[!ht]
\centerline{\includegraphics[scale=0.7]{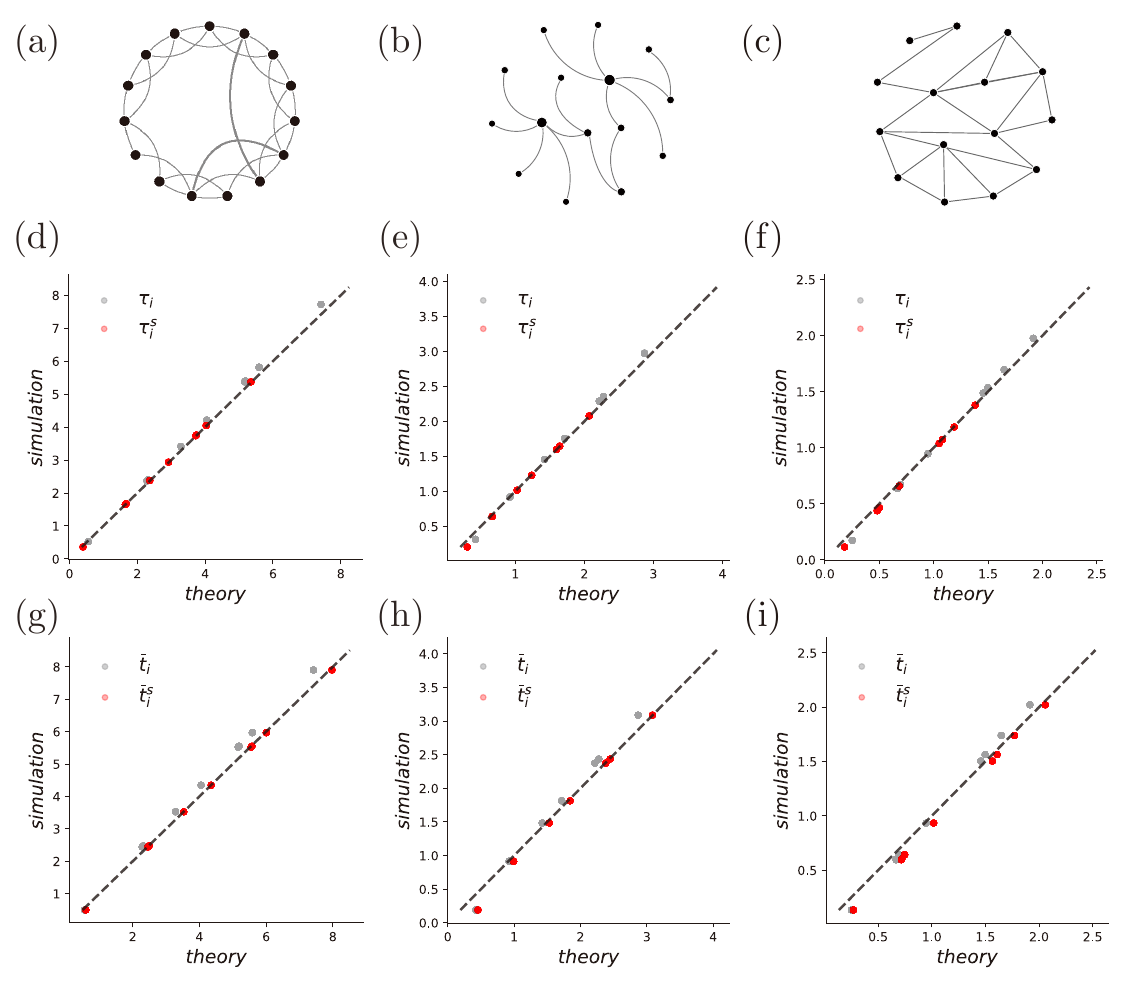}}
    \caption{
Constant perturbation spreading through small-world, scale-free, and geometric networks ($N=100$ nodes). Each network type simulated for $100$ rounds with random node perturbation. NSDD parameters: $\alpha = 1$ (edge weights), $\beta = 1$ (self-decay). (a) Small-world network sketch: initial ring with connections to $2$ nearest neighbors, edge rewiring probability $0.5$. (b) Scale-free network sketch: each new node attaches via $1$ edge to existing nodes. (c) Geometric network sketch: edges created between nodes within distance threshold $0.2$. (d-f) Simulated vs. theoretical time constants for exponential ($\tau_i$) and sigmoidal ($\tau_i^s$) functions across all rounds (small-world: d; scale-free: e; geometric: f). (g-i) Simulated vs. theoretical relative propagation times for exponential ($\bar{t}_i$) and sigmoidal ($\bar{t}_i^s$) functions across all rounds (small-world: g; scale-free: h; geometric: i).
}
\label{}
\end{figure}

\begin{figure}[!ht]
    \centerline{\includegraphics[scale=0.8]{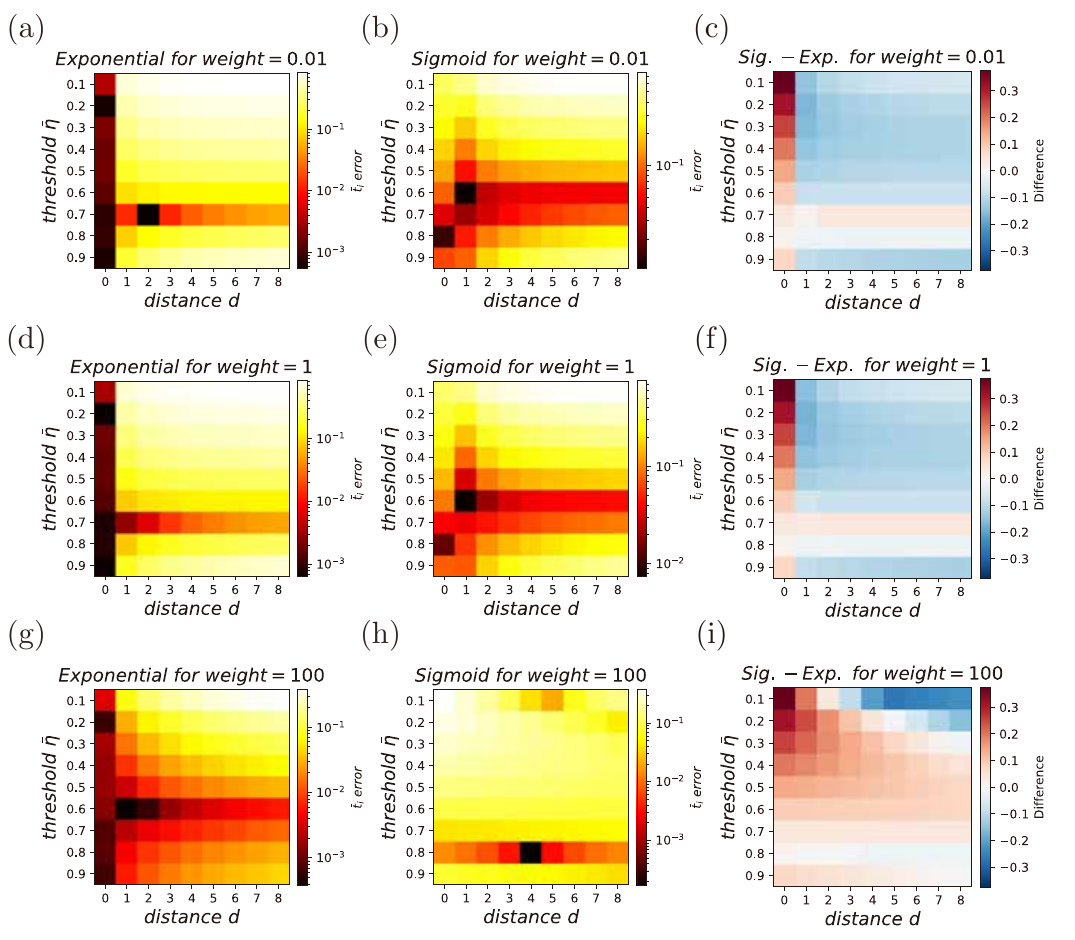}}
    \caption{
Relative error for thresholds $\bar{\eta}$ and distances $d$ at edge weights $\alpha = 0.01, 1, 100$ in a directed chain with constant inputs. The self-decay parameter $\beta = 1$. The sigmoid model yields better fits for smaller $\alpha$ values (c, f), while the exponential model is better for larger $\alpha$ (i).
}
\label{Constant_time_nine}
\end{figure}

\begin{figure}[!ht]
    \centerline{\includegraphics[scale=0.32]{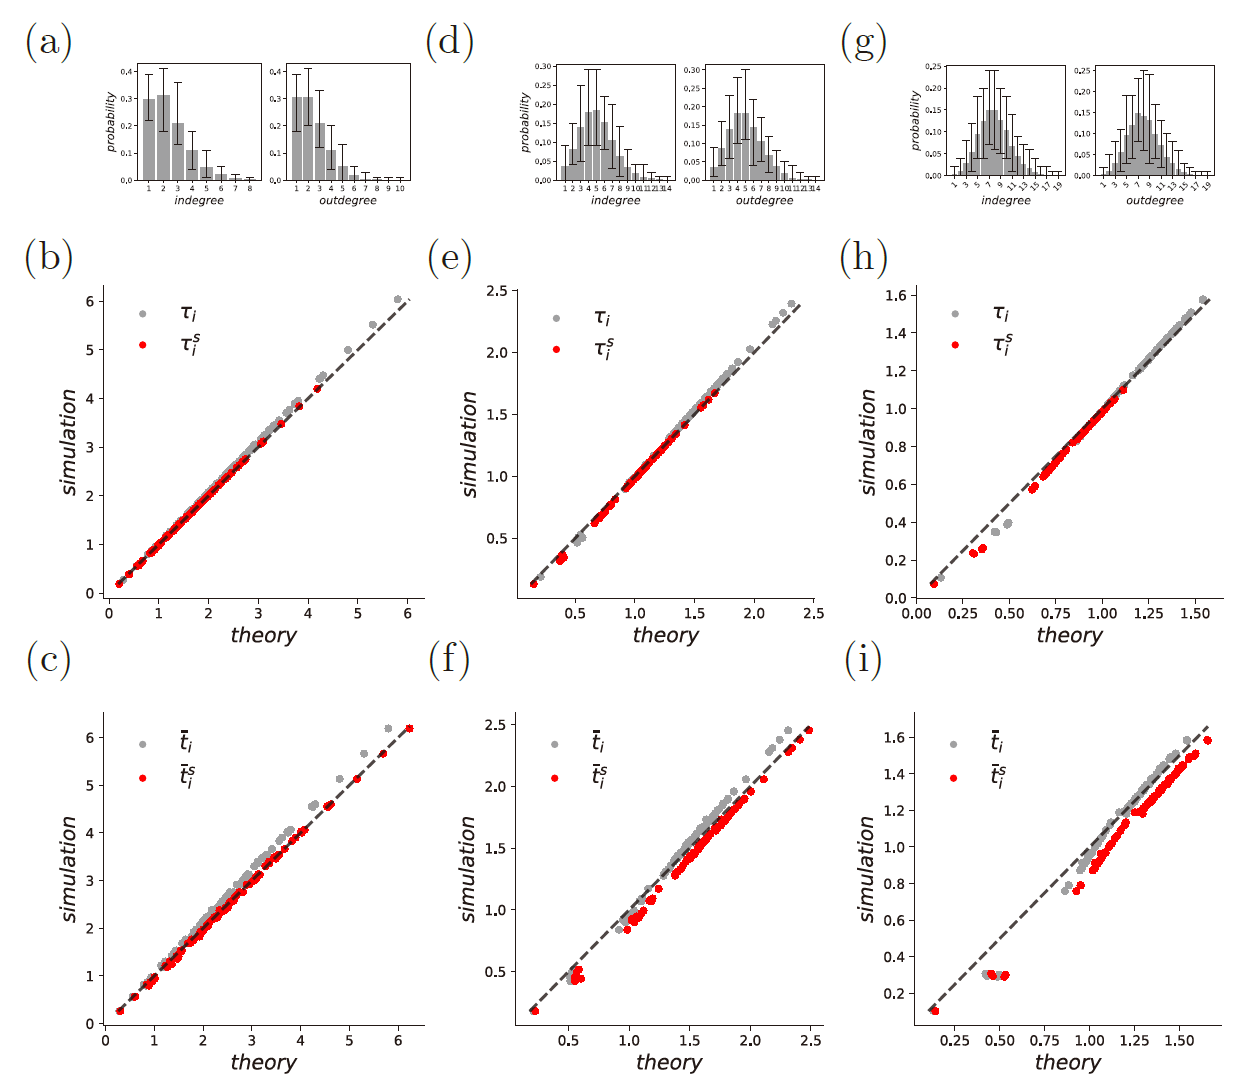}}
    \caption{Constant perturbation spreads through in the ER random networks with different edge connecting probability. Results for probability $0.02$ (a-c), $0.05$ (d-f), and $0.08$ (g-i). (a,d,g) Degree distribution for in-degree and out-degree. (b,e,h) Comparison between simulated and theoretical results for time constants for both exponential ($\tau_i$) and sigmoidal ($\tau_i^s$) functions for all rounds. (c,f,i) Comparison between simulated and theoretical results for relative time for both exponential ($\bar{t}_i$) and sigmoidal ($\bar{t}_i^s$) functions for all rounds. All theoretical results fit well with the simulated results.}
\label{constant_random_more_p}
\end{figure}

\begin{figure}[!ht]
    \centerline{\includegraphics[scale=0.6]{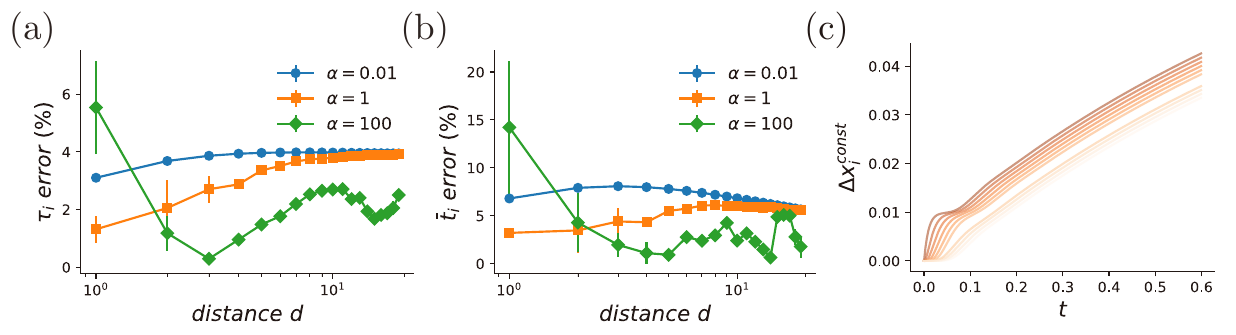}}
    \caption{
Relative error analysis for constant perturbation in Erdős-Rényi random networks ($p=0.02$) with different interaction weights. (a) Time constant ($\tau$) relative error at $\alpha = 0.01, 1, 100$. (b) Propagation time relative error at the threshold $\bar{\eta} = 1-1/e$ for $\alpha = 0.01, 1, 100$. (c) Time courses at large $\alpha$ ($100$): flat curve segment corresponds to multi-peak impulse response (Fig. \ref{pulse_error}); estimations maintain high accuracy despite this feature.
}
\label{constant_error}
\end{figure}
\clearpage

\subsection{Pulse input}
\label{supp:pulse}
\begin{figure}[!ht]
\centerline{\includegraphics[scale=0.7]{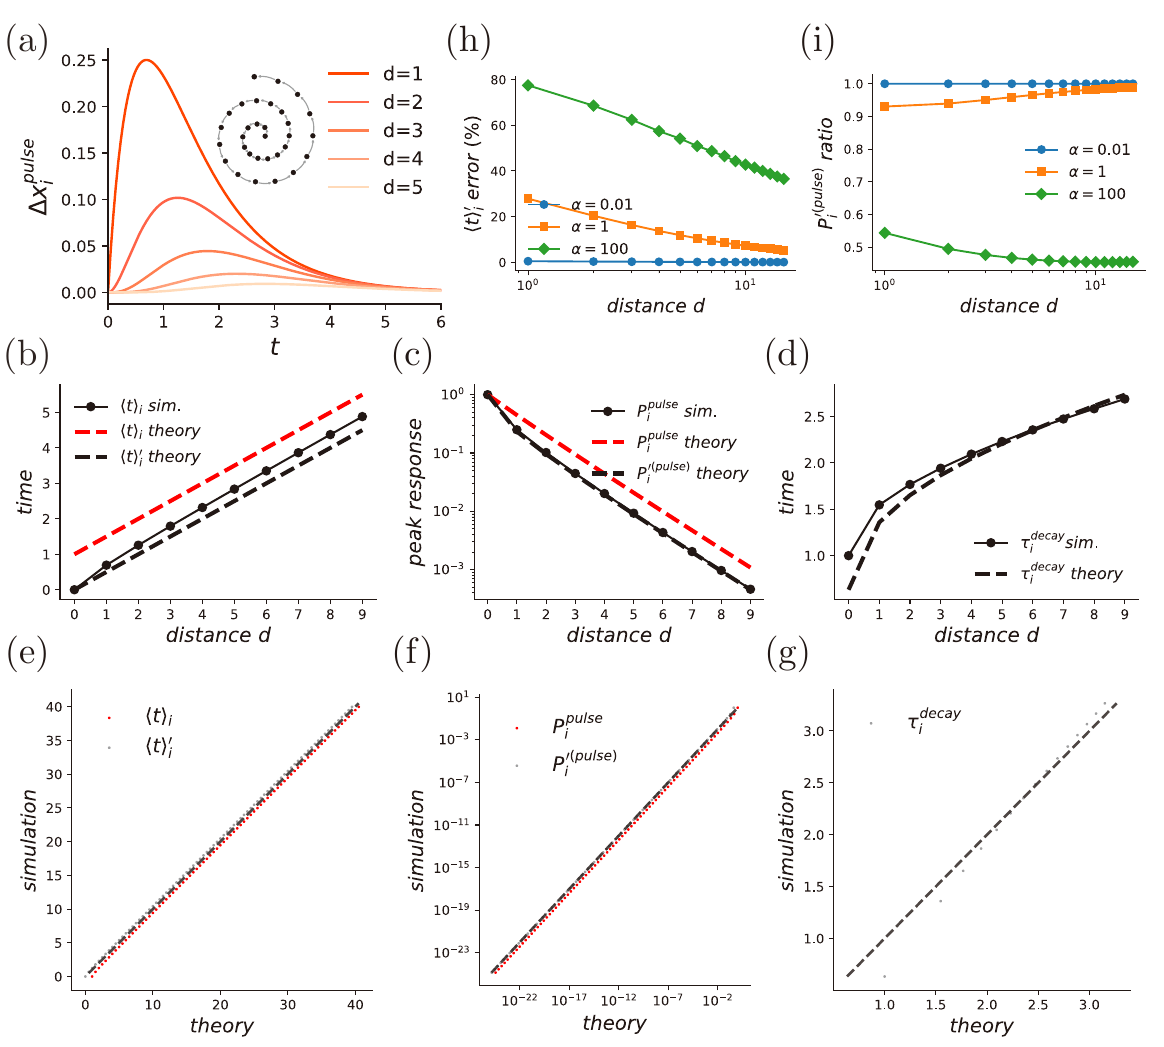}}
    \caption{
Impulse response in a directed chain ($N=80$). NSDD parameters: $\alpha = 1$, $\beta = 1$ (panels a-g). (a) Time course vs. shortest path length from input. (b) Peak response time vs. path length $d$: simulated results vs. theoretical predictions vs. amended predictions. (c) Peak response vs. path length $d$: simulated results vs. theoretical predictions vs. amended predictions. (d) Simulated vs. theoretical decay time constants. (e) Simulated vs. theoretical and amended peak response time. (f) Simulated vs. theoretical and amended peak response. (g) Simulated decay time constants vs. theoretical predictions for $d<15$ (differences increase with distance due to sharp decay; dashed lines: perfect matches). (h) Time constant relative error ($|\text{sim. } t - \text{thr. } t|/\text{sim. } t$) for $\alpha = 0.01, 1, 100$: error decreases with distance, minimal at smallest $\alpha$. (i) Peak response ratio ($\text{thr. } P/\text{sim. } P$) for $\alpha = 0.01, 1, 100$: ratio tends to $1$ at smallest $\alpha$.
}
\label{pulse_chain}
\end{figure}

\begin{figure}[!ht]
\centerline{\includegraphics[scale=0.36]{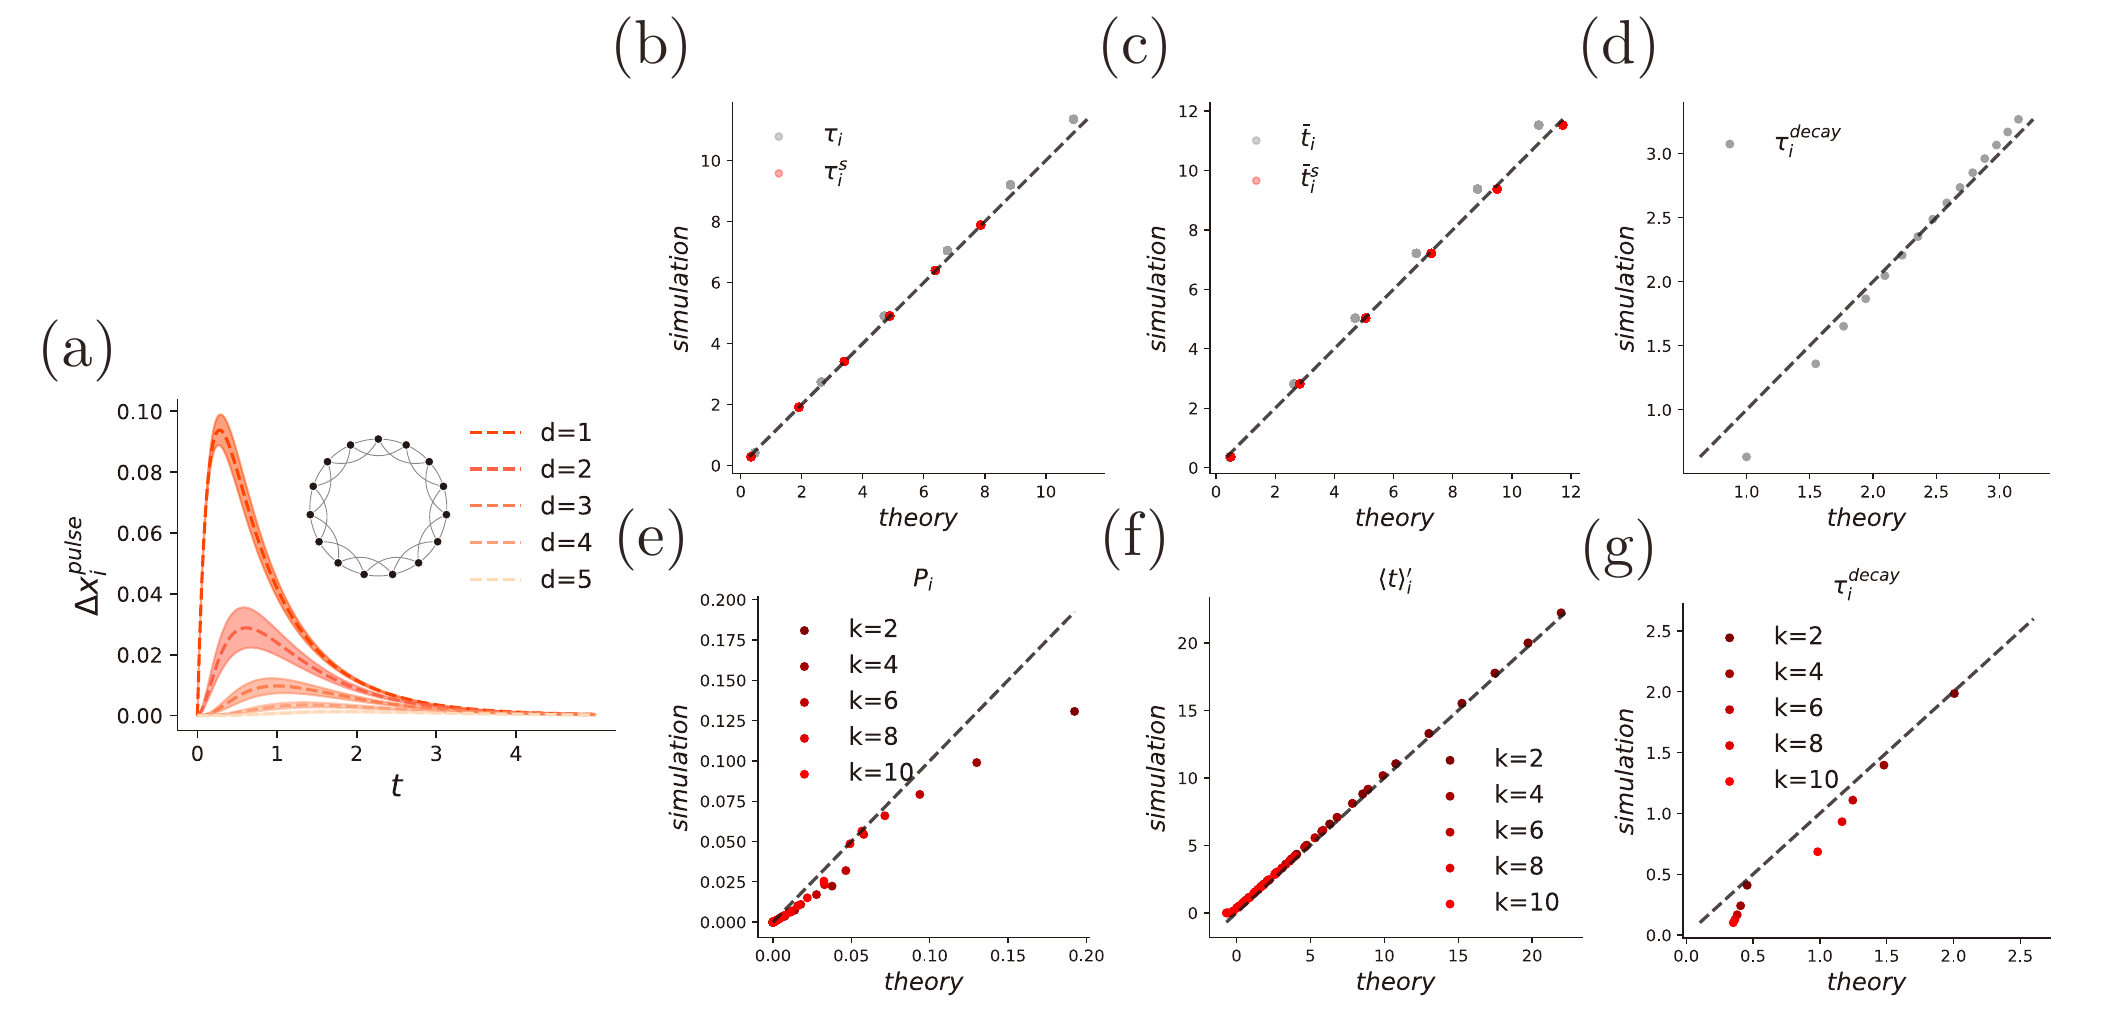}}
    \caption{
Impulse response in a ring lattice ($N=80$). NSDD parameters: $\alpha = 1$, $\beta = 1$. Node degree = 4 for panels (b)-(d). (a) Time course vs. shortest path length from input. (b) Simulated vs. theoretical and amended peak response. (c) Simulated vs. theoretical and amended peak response time. (d) Simulated decay time constants vs. theoretical predictions. (e) Simulated vs. theoretical amended peak response across different node degrees (bias increases with degree). (f) Simulated vs. theoretical amended peak response time across different node degrees. (g) Simulated decay time constants vs. theoretical predictions across different node degrees.
}
\label{pulse_regular}
\end{figure}

\begin{figure}[!ht]
\centerline{\includegraphics[scale=0.5]{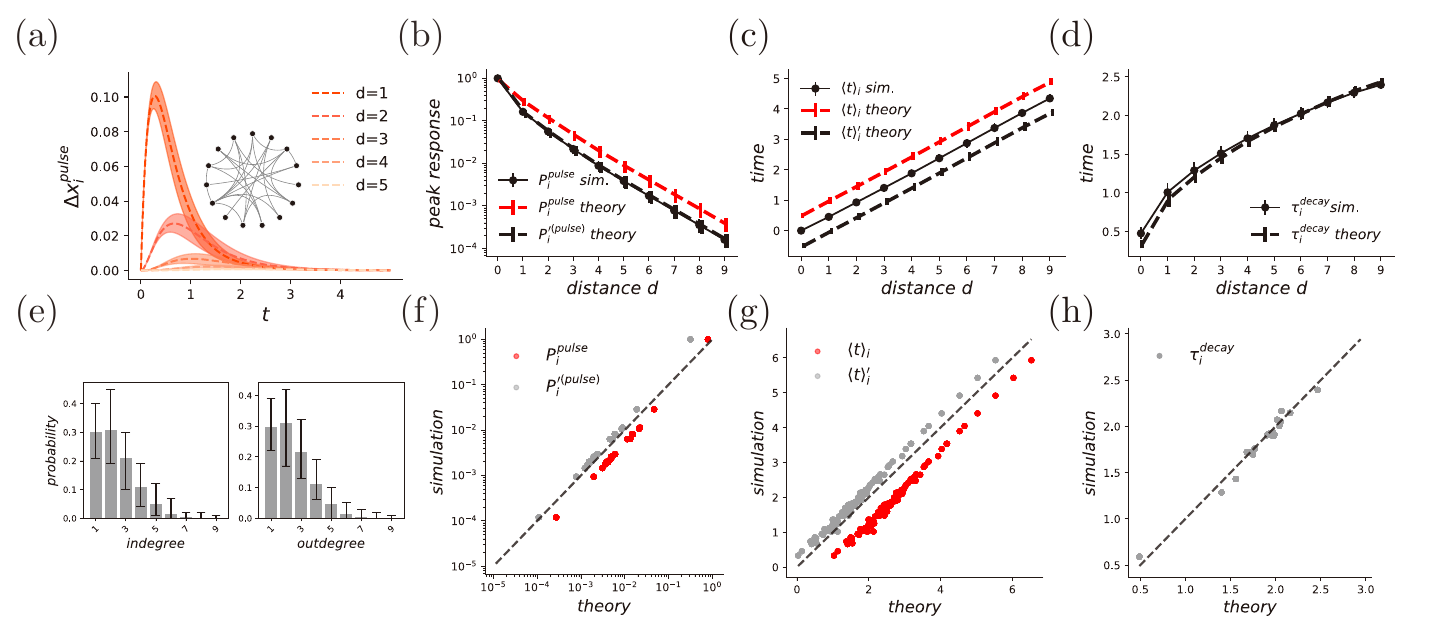}}
    \caption{
Impulse response in an Erdős-Rényi random network ($N=80$). Results from $100$ simulation rounds with NSDD parameters: $\alpha = 1$, $\beta = 1$. (a) Time course vs. shortest path length from input. (b) Peak response vs. path length $d$: simulated results vs. theoretical predictions vs. amended predictions. (vertical lines: error ranges). (c) Peak response time vs. path length $d$: simulated results vs. theoretical predictions vs. amended predictions. (simulations lie between initial and amended predictions). (d) Simulated decay time constants vs. theoretical predictions. (e) In-degree and out-degree distributions. (f) Simulated vs. theoretical and amended peak response across all rounds. (g) Simulated vs. theoretical and amended peak response time across all rounds. (h) Simulated decay time constants vs. theoretical predictions across all rounds.
}
\label{pulse_random}
\end{figure}

\begin{figure}[!ht]
\centerline{\includegraphics[scale=0.55]{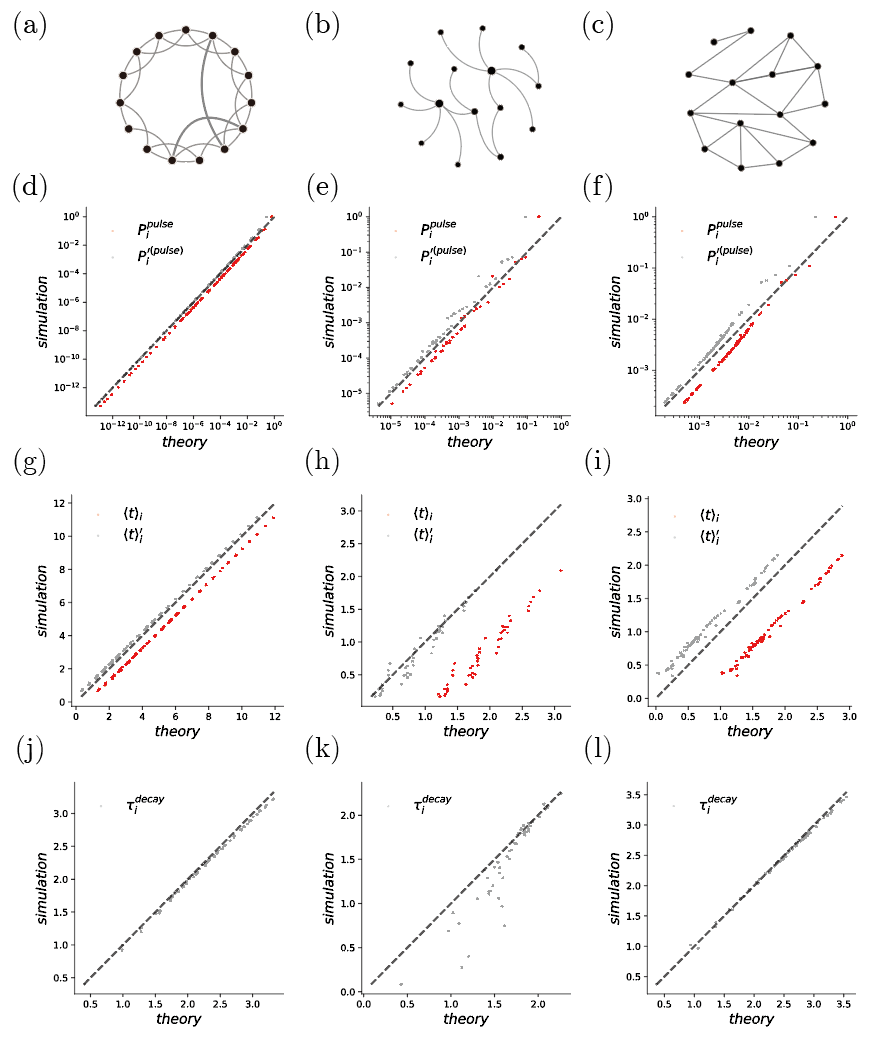}}
    \caption{
Pulse perturbation in small-world, scale-free, and geometric networks ($N=100$). Each network simulated for $100$ rounds. NSDD parameters: $\alpha = 1$, $\beta = 1$. (a) Small-world sketch: initial ring with connections to $2$ nearest neighbors, edge rewiring probability $0.5$. (b) Scale-free sketch: each new node attaches via $1$ edge to existing nodes. (c) Geometric sketch: edges created between nodes within distance threshold $0.2$. (d-f) Simulated vs. theoretical peak response for initial theory ($P_i^{\text{pulse}}$) and amended theory ($P_i^{\prime\text{(pulse)}}$) across all rounds (d: small-world; e: scale-free; f: geometric). (g-i) Simulated vs. theoretical peak response time for initial theory ($\langle t\rangle^{\prime}_i$) and amended theory ($\langle t\rangle_i$) across all rounds (g: small-world; h: scale-free; i: geometric). (j-l) Simulated vs. theoretical peak response time from decay time constant ($\tau_i^{\text{decay}}$) across all rounds (j: small-world; k: scale-free; l: geometric).
}
\label{pulse_other}
\end{figure}

\begin{figure}[!ht]
    \centerline{\includegraphics[scale=0.42]{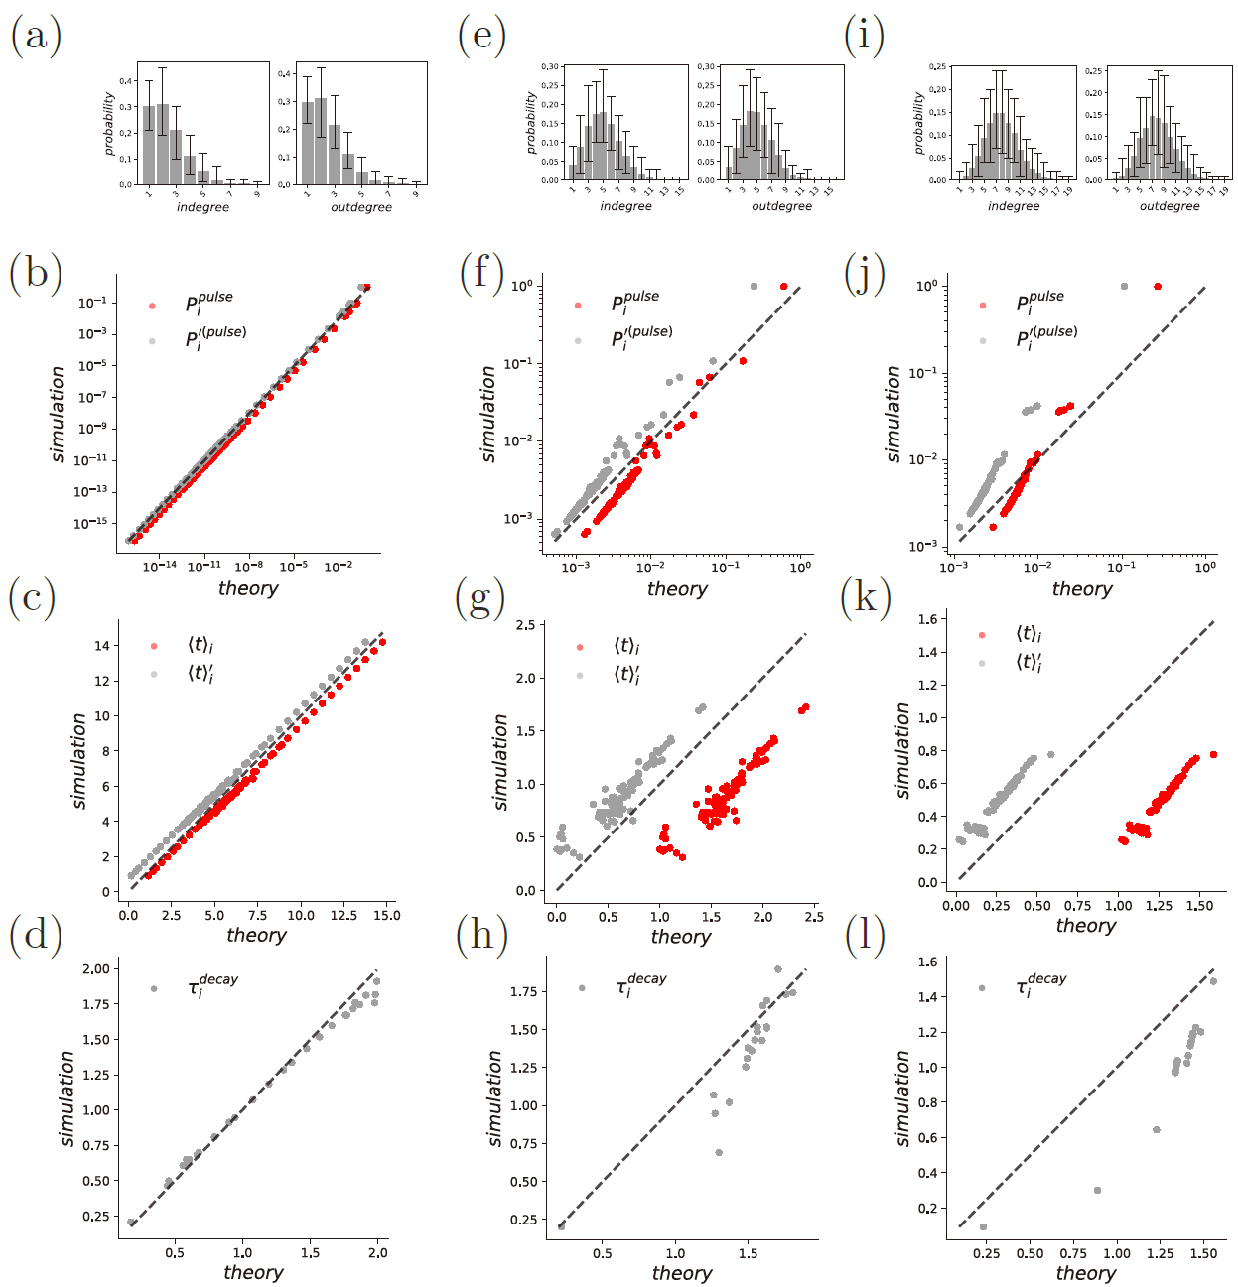}}
    \caption{
Pulse perturbation in Erdős-Rényi random networks with edge probabilities $p=0.02$ (a-d), $p=0.05$ (e-h), and $p=0.08$ (i-l). (a,e,i) In-degree and out-degree distributions. (b,f,j) Simulated vs. theoretical peak response for initial ($P_i^{\text{pulse}}$) and amended ($P_i^{\prime\text{(pulse)}}$) theories across all rounds. (c,g,k) Simulated vs. theoretical peak response time for initial ($\langle t\rangle^{\prime}_i$) and amended ($\langle t\rangle_i$) theories across all rounds. (d,h,l) Simulated decay time constants vs. theoretical predictions ($\tau_i^{\text{decay}}$) across all rounds. At higher $p$ values (e.g., $0.08$), theoretical predictions show systematic deviations: peak responses exhibit fixed-slope discrepancies and decay time constants are overestimated.
}
\label{pulse_random_more_p}
\end{figure}

\begin{figure}[!ht]
    \centerline{\includegraphics[scale=0.7]{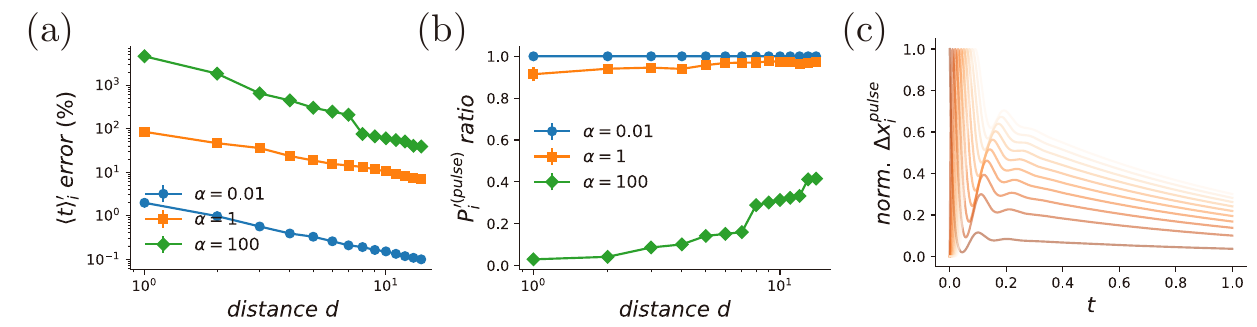}}
\caption{
Estimation error for pulse perturbation in Erdős-Rényi random networks ($p=0.02$) at edge weights $\alpha = 0.01, 1, 100$. (a) Peak response time relative error: increases with $\alpha$ (largest at $\alpha=100$). (b) Peak response ratio (theoretical/simulated): decreases with $\alpha$ (smallest at $\alpha=100$). (c) Time course at $\alpha=100$: recurrent loops generate multi-peak responses where estimations fail.
}
\label{pulse_error}
\end{figure}

\begin{figure}[!ht]
    \centerline{\includegraphics[scale=0.88]{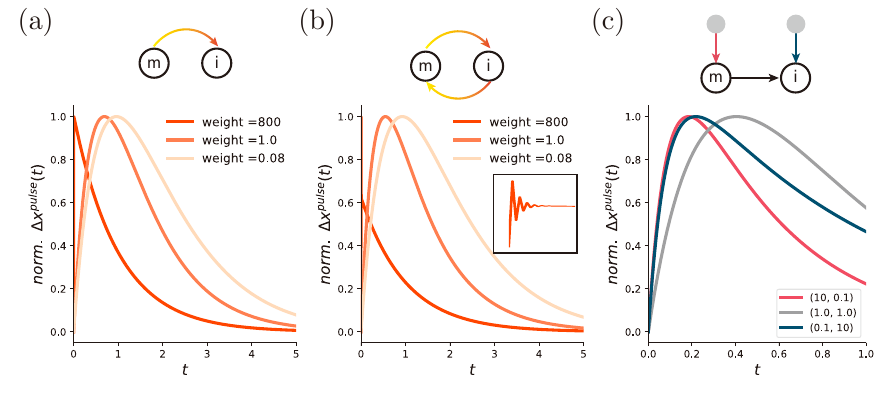}}
    \caption{
Toy model illustrating combined effects of topology, interaction weight, and degree heterogeneity. (a) Two-node directed chain: large interaction weights ($\alpha$) create significant asymmetry, explaining peak response time estimation errors at high $\alpha$ due to distribution skewness. (b) Two-node bidirectional chain: asymmetry-induced bias with damped oscillations affects peak response time estimation accuracy. (c) Degree heterogeneity effect: constant in-degree product maintained; greater heterogeneity increases asymmetry, explaining reduced estimation accuracy in scale-free networks.
}
\label{pulse_toy}
\end{figure}

\begin{figure}[!ht]
    \centerline{\includegraphics[scale=0.48]{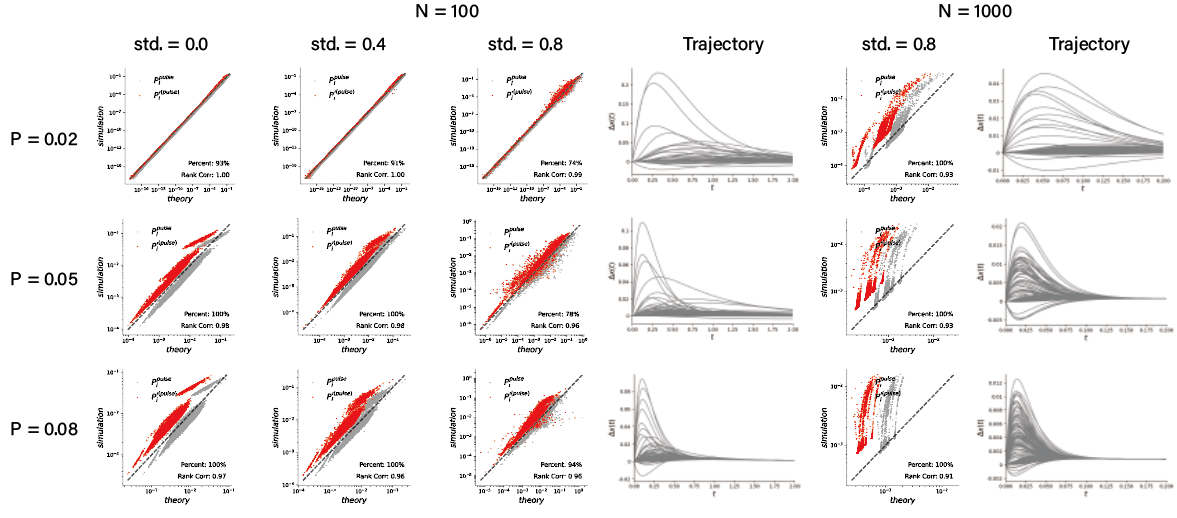}}
    \caption{
Peak response for pulse perturbation in Erdős-Rényi random networks with Gaussian weight distributions (mean = $1.0$) at different standard deviations. Network sizes: $100$ and $1000$ nodes. Edge probabilities: $0.02$ (first row), $0.05$ (second row), $0.08$ (third row). Simulated vs. theoretical extended relative time comparisons for exponential ($\bar{t}_i$) and sigmoidal ($\bar{t}_i^s$) functions over $100$ rounds. Key observations: (1) Theoretical estimates match simulations closely in dense networks (higher average degrees). (2) For larger networks (size $1000$), simulated results consistently exceed estimates. (3) At std. = $0.8$, negative weights distort nodal traces (especially in sparse networks); negative estimates and negligible responses excluded (inclusion percentages shown in lower-right corners).
}
\label{pulse_small_mean_peak}
\end{figure}

\begin{figure}[!ht]
    \centerline{\includegraphics[scale=0.48]{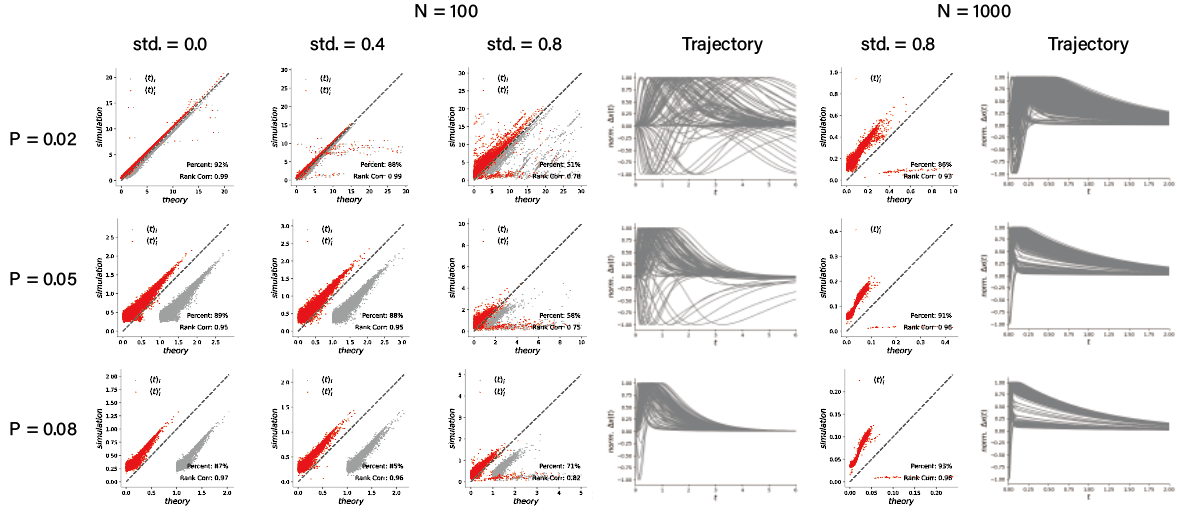}}
    \caption{Peak response time for pulse perturbation spreading in ER random networks. Networks of size $N = 100$ and $N = 1000$ with edge probabilities $p = 0.02$ (top row), $0.05$ (middle), and $0.08$ (bottom). Edge weights follow Gaussian distributions (mean $= 1.0$) with varied standard deviations. Results show extended peak response times from $100$ simulation rounds. Theoretical estimates match simulations closely in sparse networks (low $p$) without negative links. For $std. = 0.8$, negative weights significantly alter nodal traces, particularly in sparse networks. Negative theoretical values and negligible responses are excluded (inclusion percentages in bottom-right).}
\label{pulse_small_mean_time}
\end{figure}
\clearpage

\subsection{Square input}
\label{supp:square}
\begin{figure}[!ht]
    \centerline{\includegraphics[scale=0.78]{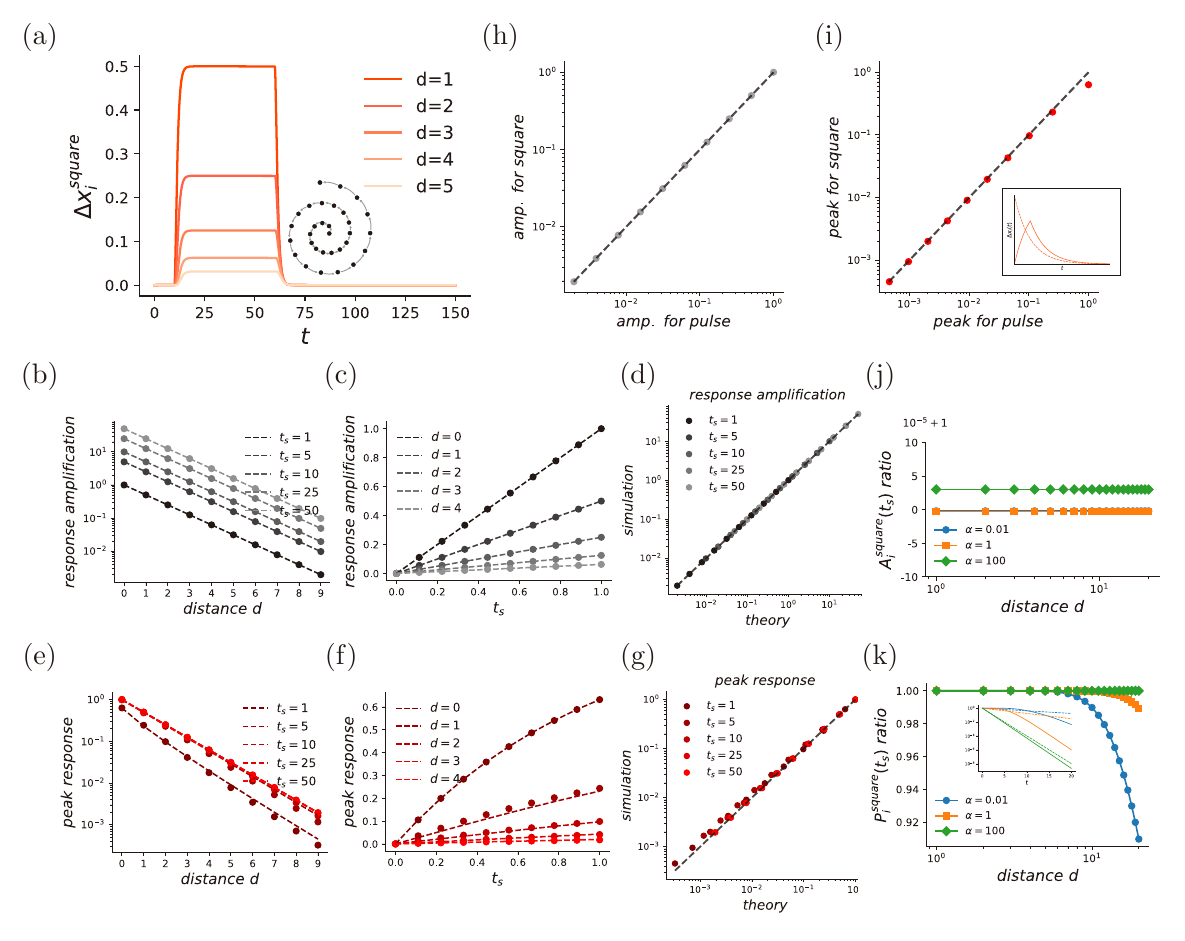}}
    \caption{Dynamics of square input propagation in a directed chain ($N=100$) with NSDD parameters ($\alpha=1$, $\beta=1$). Input is applied to the first node. 
(a) Time courses at nodes with varying distances from the source. 
(b) Response amplification vs. distance for different duration lengths ($t_s$). 
(c) Response amplification vs. $t_s$ for different distances. 
(d) Theoretical vs. simulated amplification across $t_s$. 
(e) Peak response vs. distance for different $t_s$. 
(f) Peak response vs. $t_s$ for different distances. 
(g) Theoretical vs. simulated peak response (simulations show larger peaks at small $t_s$). 
(h) Impulse response amplification matches unit-step ($t_s=1$) square input (equal input strength). 
(i) Impulse peak response aligns with unit-step input apart from the first node; inset shows response comparison at input node. 
(j) Relative error in amplification theory for $\alpha = 0.01, 1, 100$ (accurate predictions). 
(k) Theoretical/simulated peak ratio for $\alpha = 0.01, 1, 100$; deviations occur for small $\alpha$ at large distances due to early evolution effects (inset: exponential fitting).}
\label{Square_chain}
\end{figure}

\begin{figure}[!ht]
    \centerline{\includegraphics[scale=0.55]{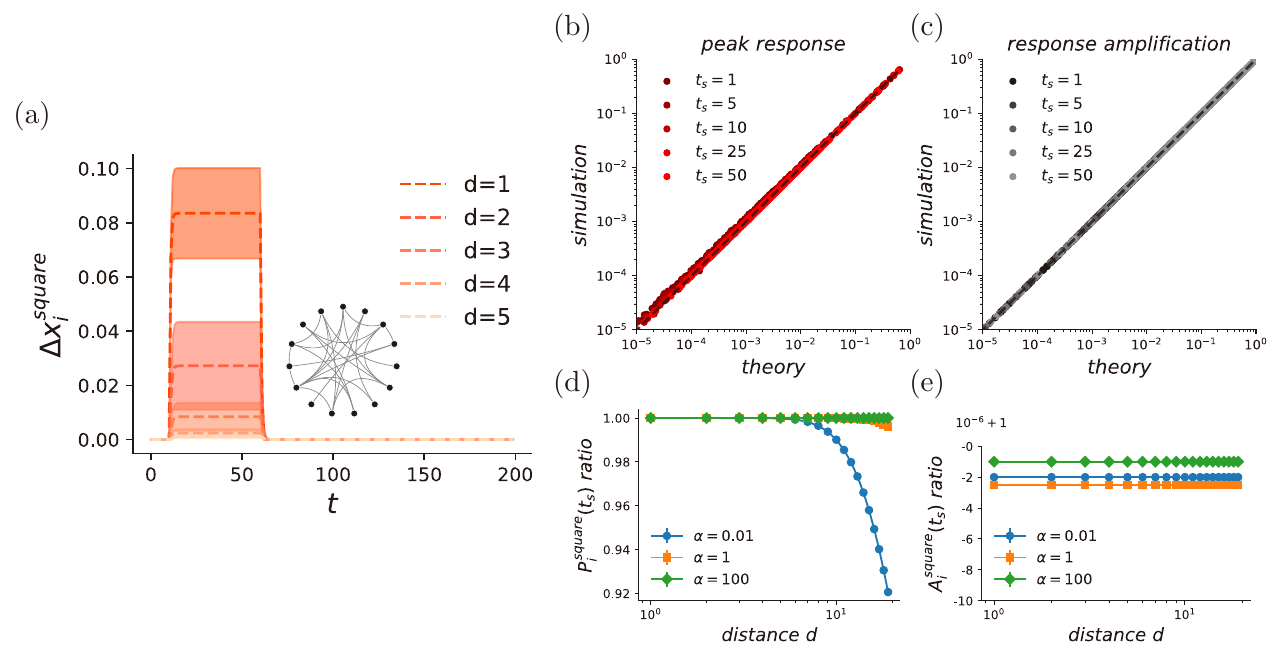}}
    \caption{Propagation dynamics of square inputs in random networks ($N=100$) with NSDD parameters ($\alpha=1$, $\beta=1$). A single input is applied at random nodes. 
(a) Time courses at varying distances from input node; shading indicates response deviations for several realizations. 
(b) Theoretical vs. simulated amplification across duration lengths ($t_s$). 
(c) Theoretical vs. simulated peak response across $t_s$. 
(d) Theoretical/simulated peak ratio (thr. P/sim. P) for $\alpha = 0.01, 1, 100$, showing deviations at small $\alpha$ and large distances. 
(e) Theoretical/simulated amplification ratio for $\alpha = 0.01, 1, 100$, demonstrating accurate estimation.}
\label{square_random}
\end{figure}

\begin{figure}[!ht]
    \centerline{\includegraphics[scale=0.65]{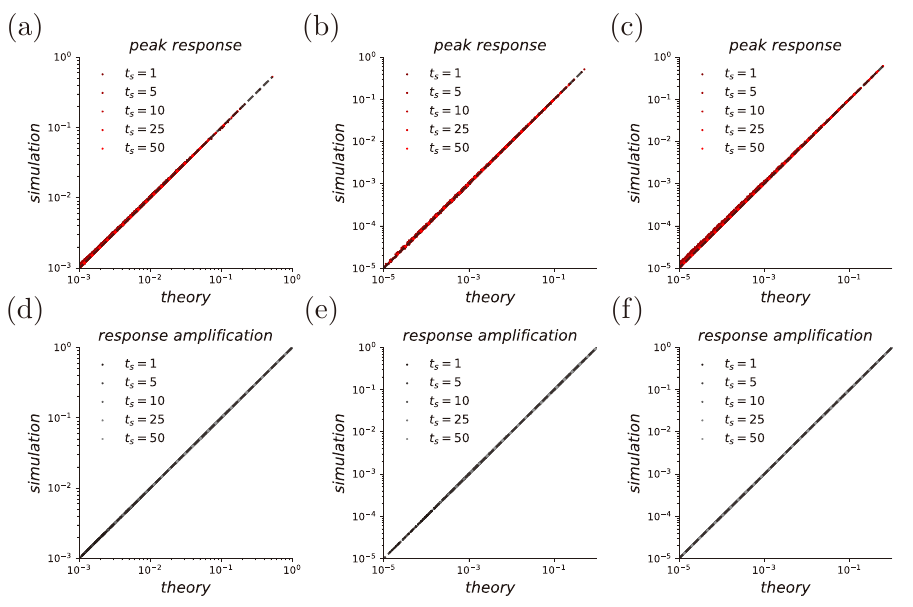}}
    \caption{Propagation dynamics of square perturbations in three networks (each $N=100$): small-world (a,d), scale-free (b,e), and geometric (c,f). All simulations use $\alpha=1$, $\beta=1$ and $100$ rounds, with any single-node inputs. Network specifications: (a,d) Small-world: Initial ring with $2$ nearest neighbors per node, edge rewiring probability $0.5$; (b,e) Scale-free: Preferential attachment ($1$ edge per new node); (c,f) Geometric: Edge creation threshold radius $0.2$. Panels show theoretical estimations of (a-c) peak response and (d-f) response amplification.}
\label{square_other}
\end{figure}
\clearpage

\subsection{Noise input}
\label{supp:noise}

\begin{figure}[!ht]
    \centerline{\includegraphics[scale=0.5]{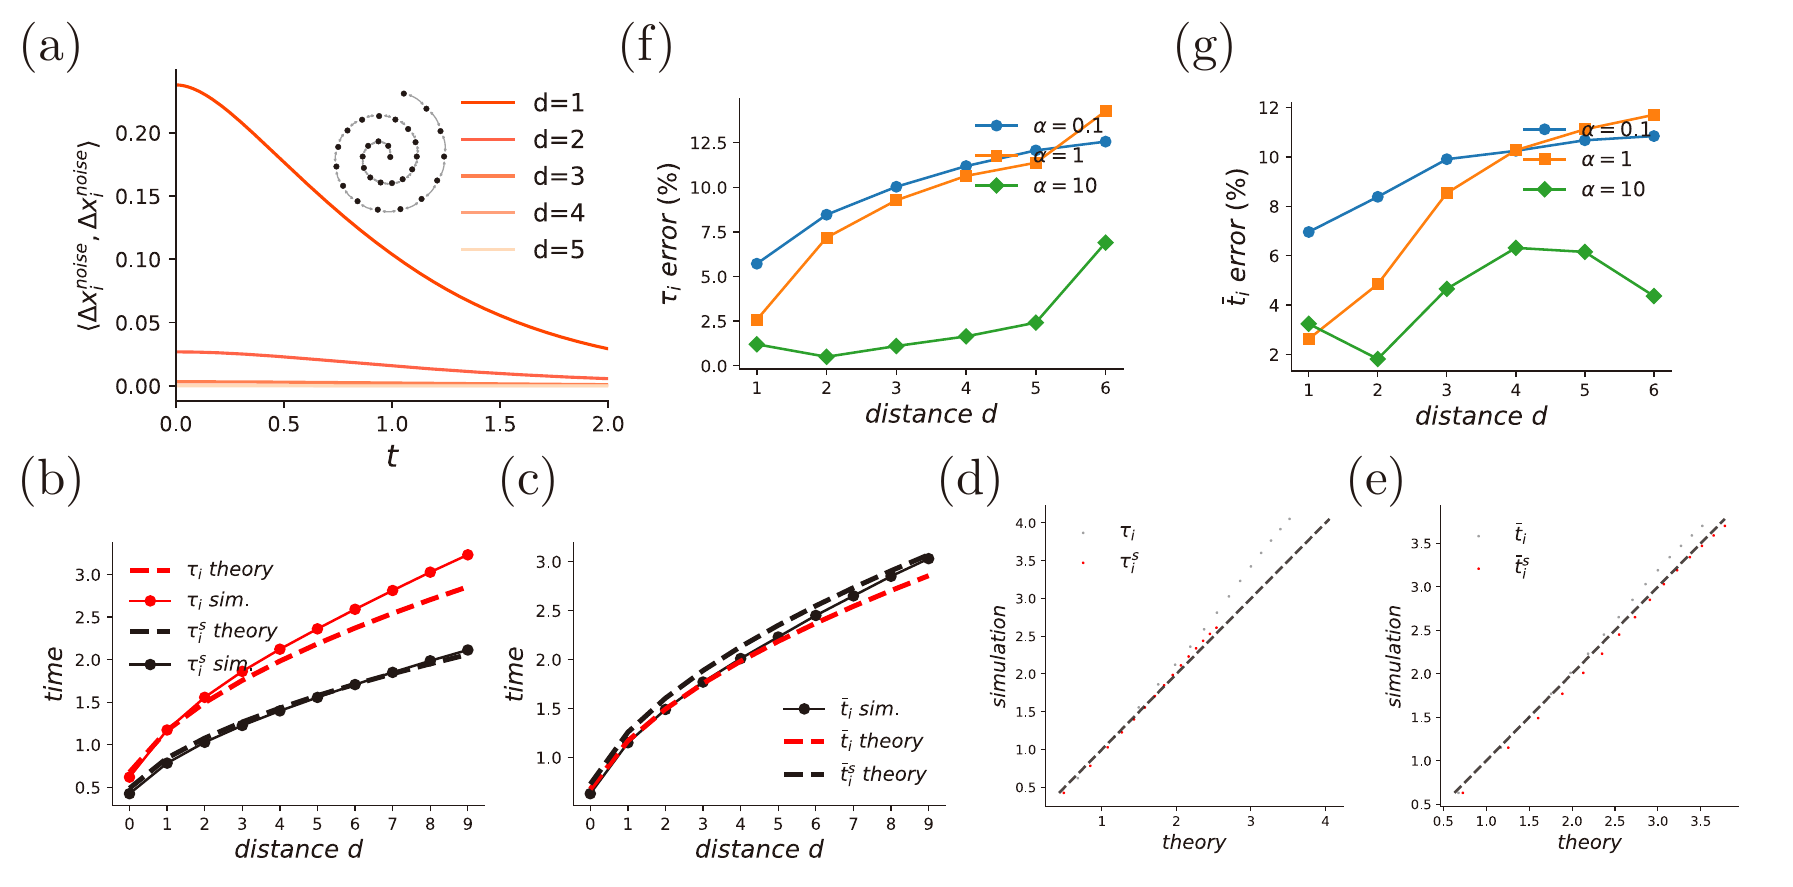}}
    \caption{White noise response dynamics in an undirected chain ($N=100$) with NSDD parameters ($\alpha=1$, $\beta=1$). Input targets the first node. Threshold $\bar{\eta} = 1/e$ applies to panels (c,e,g). 
(a) Autocovariance dynamics for different shortest path distance $d$ from input node. 
(b) Simulated and theoretical time constant with exponential form $\tau_i$ and sigmoidal form $\tau_i^s$ vs. distance $d$. 
(c) Simulated and theoretical relative propagation time with exponential form $\bar{t}_{i}$ and sigmoidal form $\bar{t}_{i}^s$ vs. distance $d$. 
(d) Theoretical vs. simulated time constants (initial/amended). 
(e) Theoretical vs. simulated relative propagation times (initial/amended). 
(f) Relative error of $\tau$ ($|\text{sim.} - \text{thr.}|/\text{sim.}$) for $\alpha = 0.1, 1, 10$: error increases with $d$ and minimizes at largest $\alpha$. 
(g) Relative error of $\bar{t}_{i}$ for $\alpha = 0.1, 1, 10$: similar trend as (f).}
\label{auto_chain}
\end{figure}

\begin{figure}[!ht]
    \centerline{\includegraphics[scale=0.44]{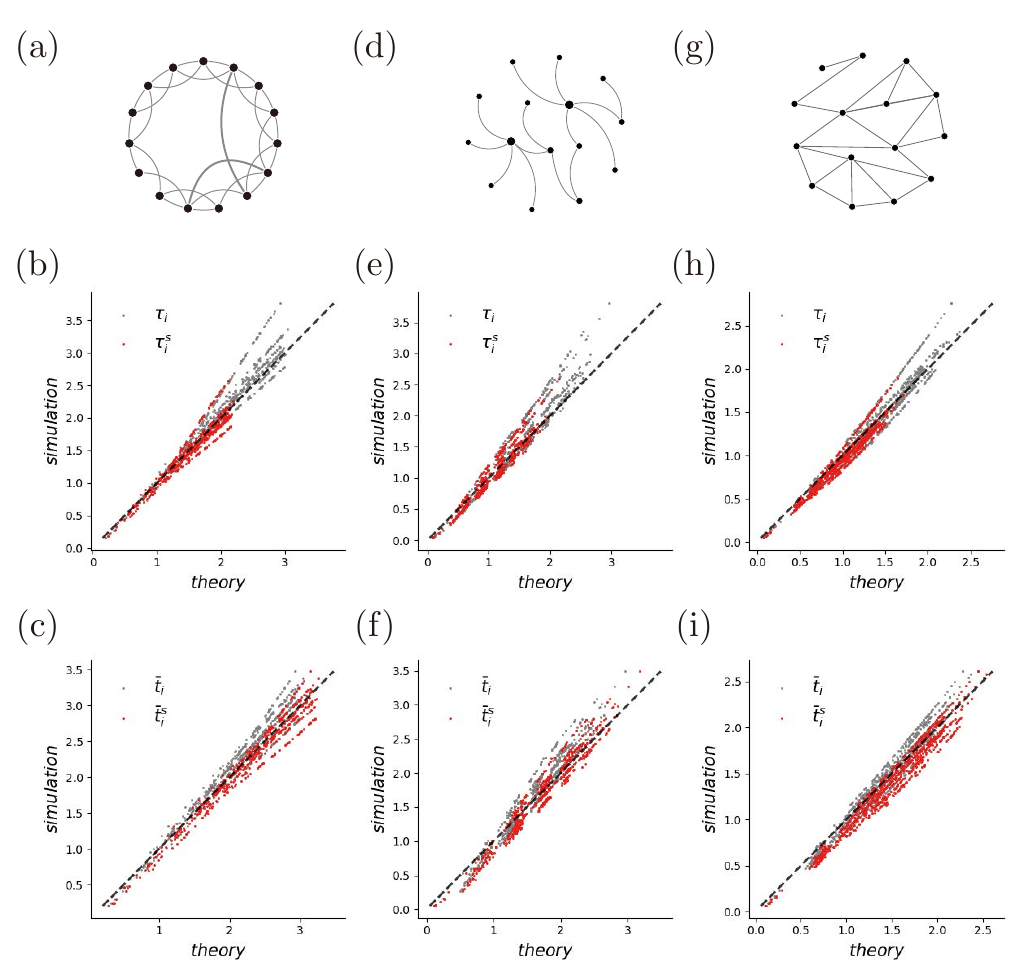}}
    \caption{Autocovariance dynamics of white noise perturbations in three networks: small-world (a-c), scale-free (d-f), and geometric (g-i). Simulations use $N=100$, NSDD parameters ($\alpha=1$, $\beta=1$), with $10$ random network instances each run for $10$ rounds. Single-node perturbations applied randomly. Network schematics: Small-world: initial ring with $2$ nearest neighbors, edge rewiring probability $0.5$; Scale-free: preferential attachment ($1$ edge per new node); Geometric: connection radius threshold $0.2$; (d-f) Time constant comparison: Theoretical vs. simulated values for exponential ($\tau_i$) and sigmoidal ($\tau_i^s$) models across all networks and rounds; (g-i) Relative propagation time comparison: Theoretical vs. simulated values for exponential ($\bar{t}_i$) and sigmoidal ($\bar{t}_i^s$) models at threshold $\bar{\eta} = 1/e$}
\label{noise_auto_other}
\end{figure}

\begin{figure}[!ht]
    \centerline{\includegraphics[scale=0.5]{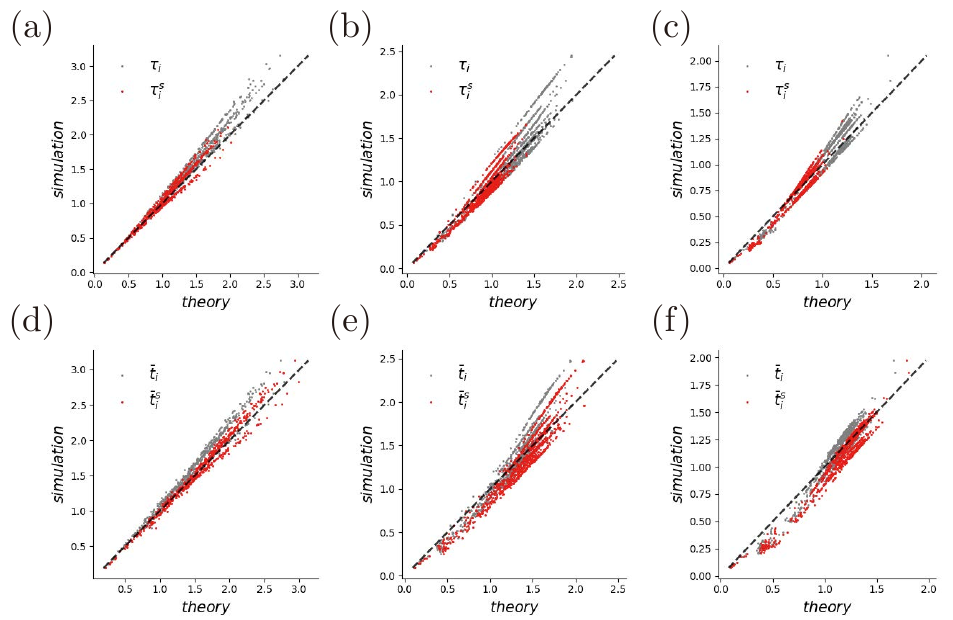}}
    \caption{Auto-covariance dynamics of white noise perturbations in ER random networks with varying edge probabilities $p$. Results compare simulations and theory for: $p = 0.02$ (a, d); $p = 0.05$ (b, e); $p = 0.08$ (c, f). (a-c) Time constants: theoretical vs. simulated for exponential ($\tau_i$) and sigmoidal ($\tau_i^s$) forms; (d-f) Relative propagation times: theoretical vs. simulated for exponential ($\bar{t}_i$) and sigmoidal ($\bar{t}_i^s$) forms. All theoretical predictions show excellent agreement with simulations.}
\label{noise_random}
\end{figure}

\begin{figure}[!ht]
    \centerline{\includegraphics[scale=0.45]{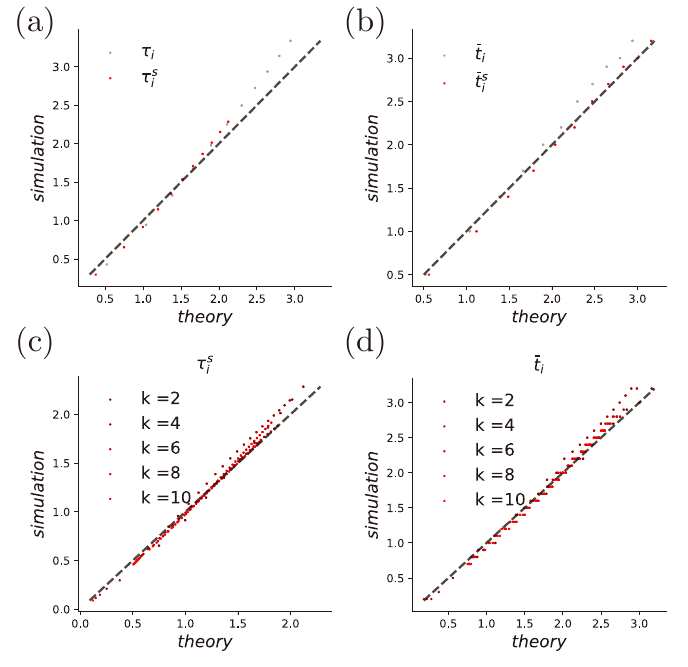}}
    \caption{White noise dynamics in a ring lattice network ($N=100$) with NSDD parameters ($\alpha=1$, $\beta=1$). Perturbations target random nodes. Threshold $\bar{\eta} = 1/e$ applies to (b,d). (a) Time constants ($\tau$): Theoretical vs. simulated for exponential ($\tau_i$) and sigmoidal ($\tau_i^s$) models (degree $k=4$); dotted lines indicate perfect match. (b) Relative propagation times ($\bar{t}$): Theoretical vs. simulated for exponential ($\bar{t}_i$) and sigmoidal ($\bar{t}_i^s$) forms ($k=4$); (c) Time constants ($\tau_i^s$): Theoretical vs. simulated across degrees $k = 2,4,6,8,10$; (d) Relative propagation times ($\bar{t}_i^s$): Theoretical vs. simulated across $k = 2,4,6,8,10$}
\label{noise_auto_regular}
\end{figure}

\begin{figure}[!ht]
    \centerline{\includegraphics[scale=0.4]{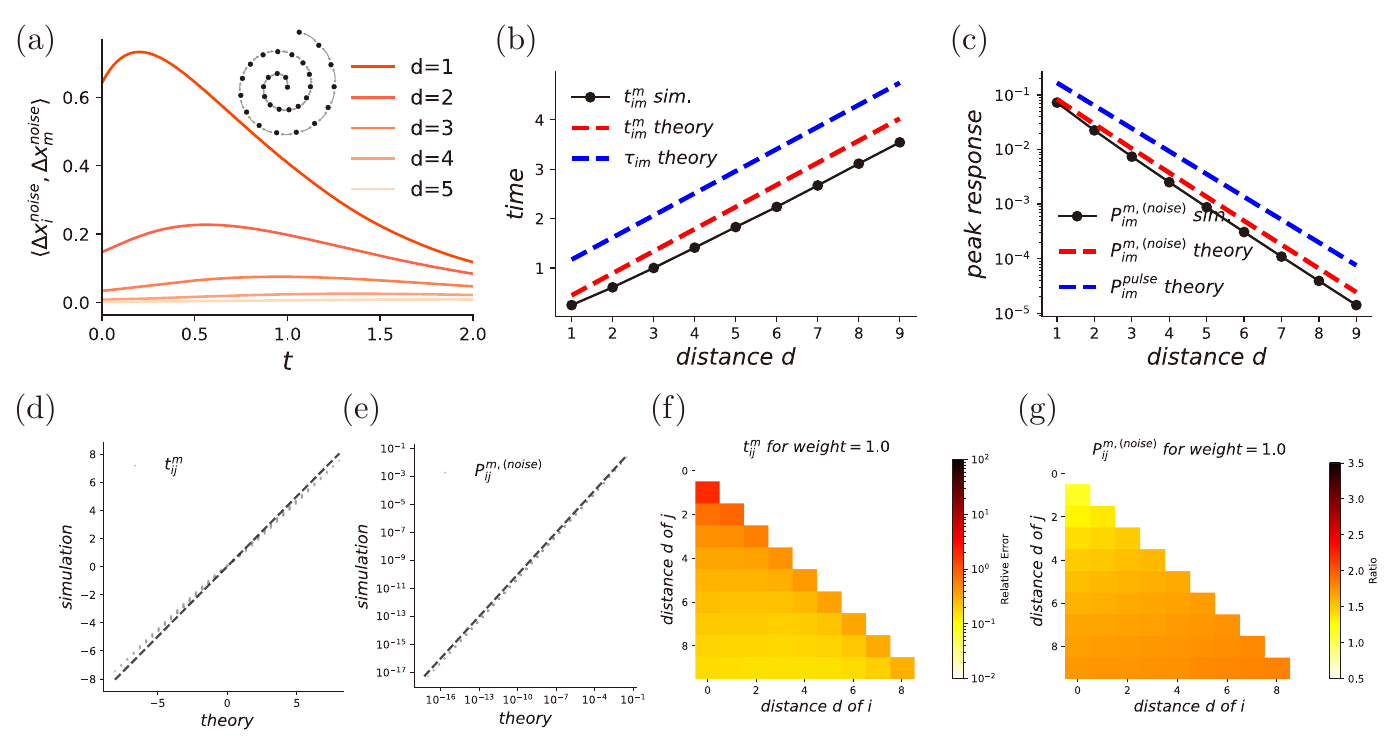}}
    \caption{White noise response dynamics in an undirected chain ($N=100$) with NSDD parameters ($\alpha=1$, $\beta=1$). Input targets the first node. Threshold $\bar{\eta} = 1/e$ applies to panels (c,e,g). (a) Crosscovariance dynamics for different shortest path distance $d$ from input node. (b) Simulated and theoretical peak times between source–target node pairs ($m,i$), denoted as $t_{im}^m$, plotted against distance $d$. The corresponding time constants $\tau_{im}$ under constant input are also shown, exhibiting trends that closely align with those of $t_{im}^m$. (c) Simulated and theoretical peak response ($P_{im}^{m,(noise)}$) vs. $d$. The corresponding peak response $P_{im}^{pulse}$ under pulse input are also shown, exhibiting trends that closely align with those of $P_{im}^{m,(noise)}$. (d) Theoretical vs. simulated peak times (initial/amended). (e) Theoretical vs. simulated peak response (initial/amended). (f) Relative error of $t_{ij}^m$ ($|\text{sim} - \text{thr}|/\text{sim}$) for node pairs $(i,j)$ when receiving input at node $m$: error increases with distance from input. (g) Peak amplitude ratio ($\text{thr } P/\text{ sim } P$) for node pairs: accuracy higher near input. Only lower half of symmetric estimation matrix shown.}
\label{cov_chain}
\end{figure}

\begin{figure}[!ht]
    \centerline{\includegraphics[scale=0.45]{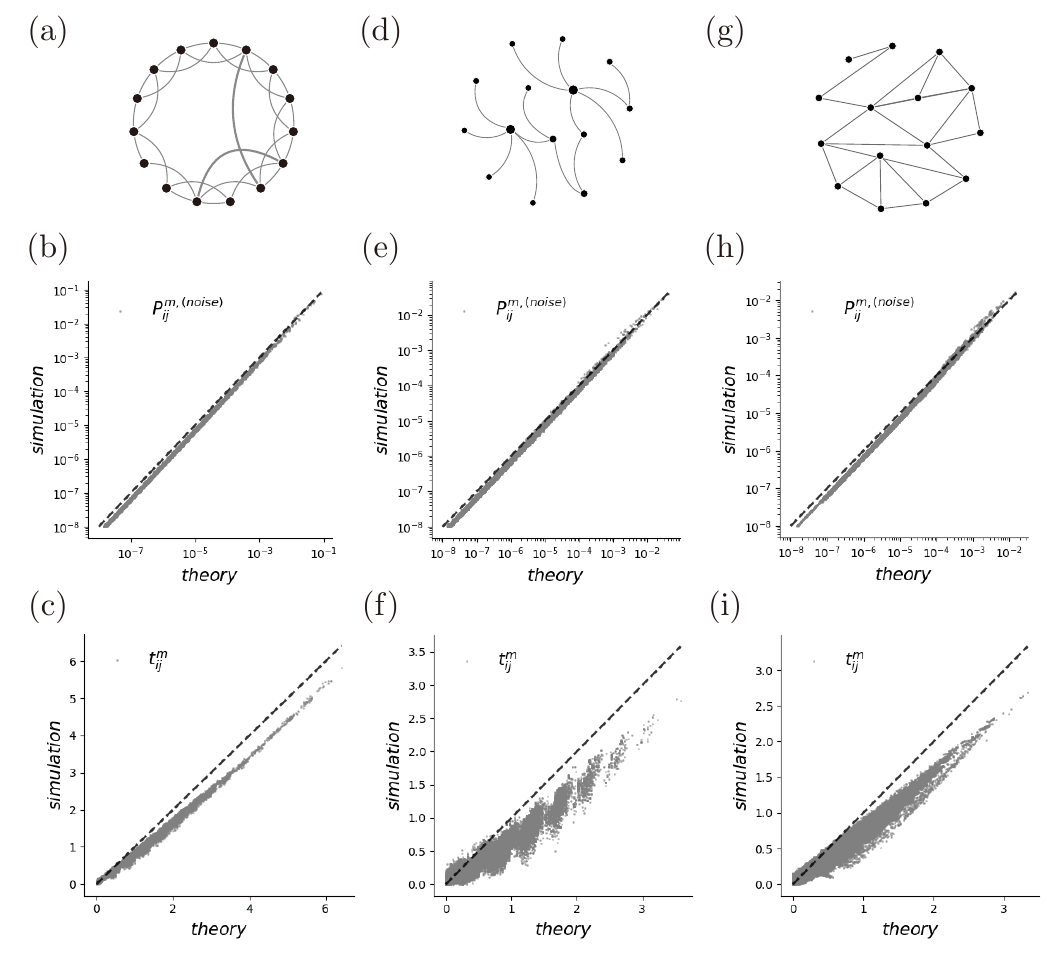}}
    \caption{Crosscovariance dynamics following white noise perturbations in three networks. Simulations use $N=100$, NSDD parameters ($\alpha=1$, $\beta=1$), with $10$ random instances per network type, each run for $10$ rounds. (a-c) Small-world schematic: initial ring with $2$ nearest neighbors, edge rewiring probability $0.5$; (d-f) Scale-free schematic: preferential attachment ($1$ edge per new node); (g-i) Geometric schematic: connection radius threshold $0.2$; (b,e,h) Peak response ($P_{ij}^{m,({noise})}$): Theoretical vs. simulated values. (c,f,i) Peak response time ($t_{ij}^m$): Theoretical vs. simulated values. Theoretical peak response time estimates are systematically higher than simulated values.}
\label{cov_other}
\end{figure}

\begin{figure}[!ht]
    \centerline{\includegraphics[scale=0.34]{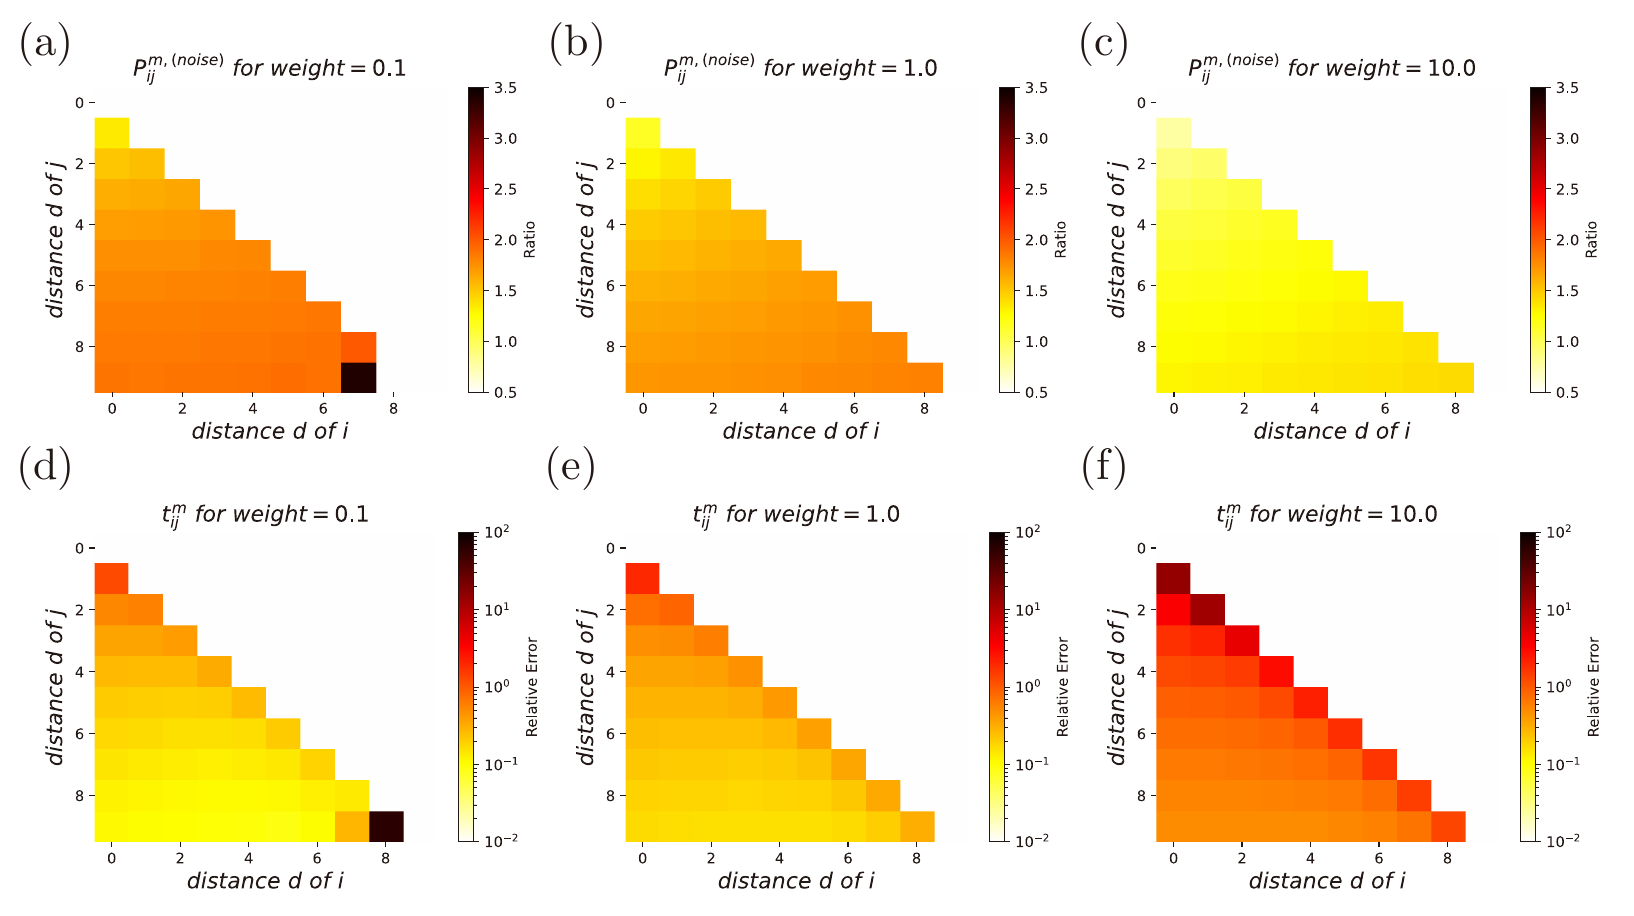}}
    \caption{Crosscovariance dynamics in an undirected chain (NSDD system, $\beta=1$) examining accuracy of peak response metrics for node pairs. Panels (a-c) show peak response ratio ($\text{thr } P/\text{ sim } P$) for interaction weights $\alpha = 0.1, 1.0, 10.0$ respectively, where accuracy improves near the input node across all weights and generally increases with higher $\alpha$ values (consistent color bar). Panels (d-f) display relative error of peak time ($|\text{sim } t - \text{thr } t|/\text{sim } t$) for $\alpha = 0.1, 1.0, 10.0$ respectively, showing improved error far from the input node, with best overall accuracy at $\alpha = 0.1$ (lightest colors in d).}
\label{cov_error}
\end{figure}

\begin{figure}[!ht]
    \centerline{\includegraphics[scale=0.75]{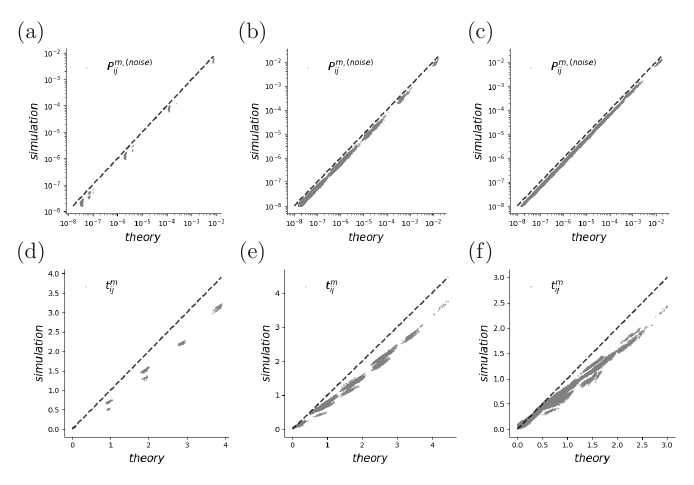}}
    \caption{White noise perturbation in ER random networks ($N=100$) with varying connecting probabilities $p$. Results for $p=0.02$ (a,d), $0.05$ (b,e), and $0.08$ (c,f) show: (a-c) Simulated vs. theoretical peak response; (d-f) Simulated vs. theoretical peak response time (theoretical estimates generally higher than simulations). For each $p$, $10$ random networks were generated and each simulated for $10$ rounds. Node pairs with distance $\geq 10$ are excluded due to significant errors.}
\label{cov_random}
\end{figure}

\begin{figure}[!ht]
    \centerline{\includegraphics[scale=0.6]{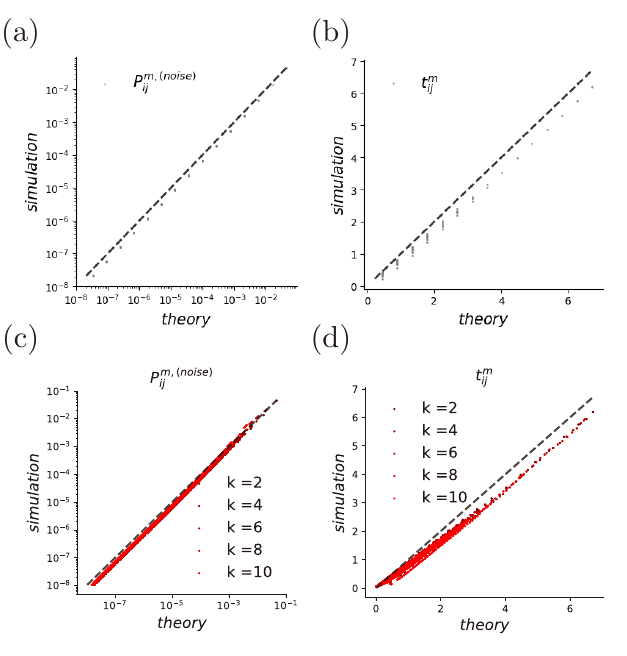}}
    \caption{White noise perturbation in a ring lattice network ($N=100$) with NSDD parameters ($\alpha=1$, $\beta=1$), targeting random nodes. Panels (a) and (b) show node degree $k=4$: (a) Simulated vs. theoretical peak response ($P_{ij}^{m,{(noise)}}$) for all node pairs (dotted lines indicate perfect agreement); (b) Simulated vs. theoretical peak response time ($t_{ij}^{m}$). Panels (c) and (d) show results across degrees $k=2,4,6,8,10$: (c) Peak response comparisons; (d) Peak response time comparisons. All panels analyze covariance between node pairs.}
\label{cov_regular}
\end{figure}

\clearpage

\section{Extension to general formalism for constant input}
\label{supp:negative}
\begin{figure}[!ht]
    \centerline{\includegraphics[scale=0.22]{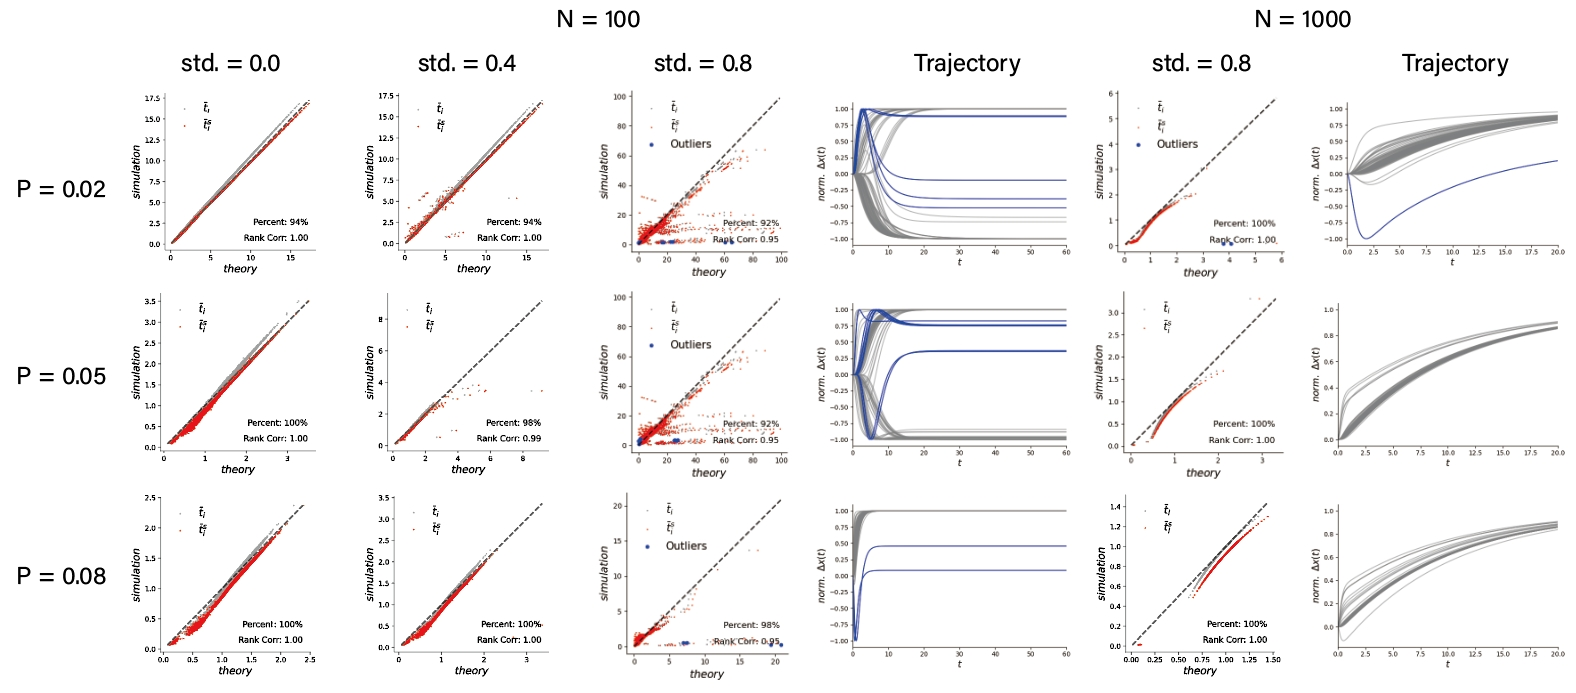}}
    \caption{Constant perturbation spreading in ER random networks with Gaussian weight distributions (mean $=1.0$). Results compare size $N=100$ vs. $1000$ and edge probabilities $p=0.02$ (top row), $0.05$ (middle), $0.08$ (bottom). Theoretical vs. simulated relative times ($\bar{t}_i$, $\bar{t}_i^s$) are shown from $100$ rounds. Theoretical estimates match simulations well in large dense networks (high average degree). For $std.=0.8$, negative weights alter nodal traces in sparse networks, causing non-monotonic traces with prominent peaks and larger theoretical estimates. Negative theoretical values and negligible responses are excluded (inclusion \% in bottom-right).}
\end{figure}

\begin{figure}[!ht]
    \centerline{\includegraphics[scale=0.22]{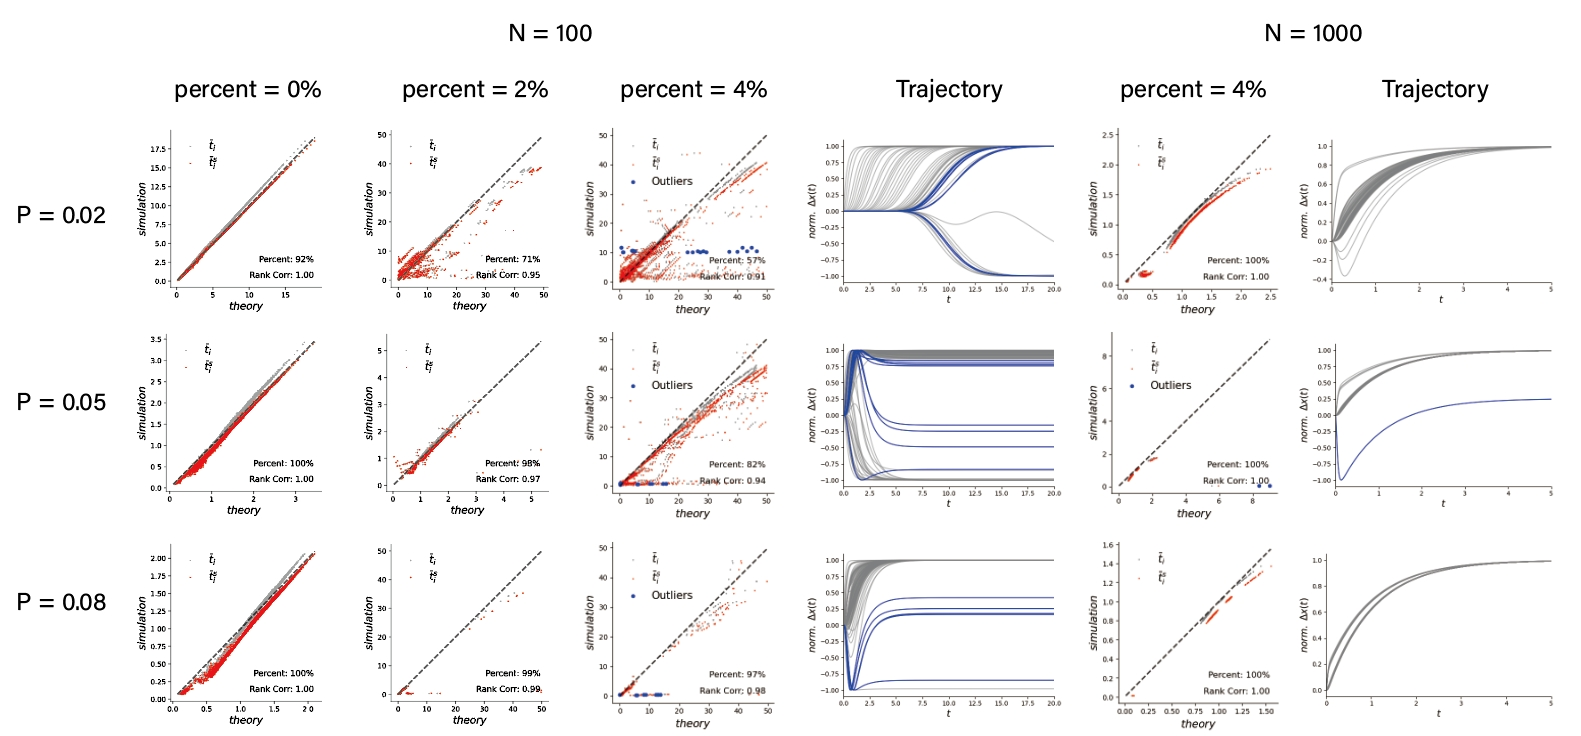}}
    \caption{Constant perturbation spreading in ER random networks with varying negative link percentages. Results compare sizes $N=100$ vs. $1000$ and negative links: $0\%$ (left column), $2\%$ (middle), $4\%$ (right). Theoretical vs. simulated relative times ($\bar{t}_i$, $\bar{t}_i^s$) from $100$ rounds show that higher negative link percentages significantly alter nodal traces, particularly in low average degree networks.}
\end{figure}

\begin{figure}[!ht]
    \centerline{\includegraphics[scale=0.23]{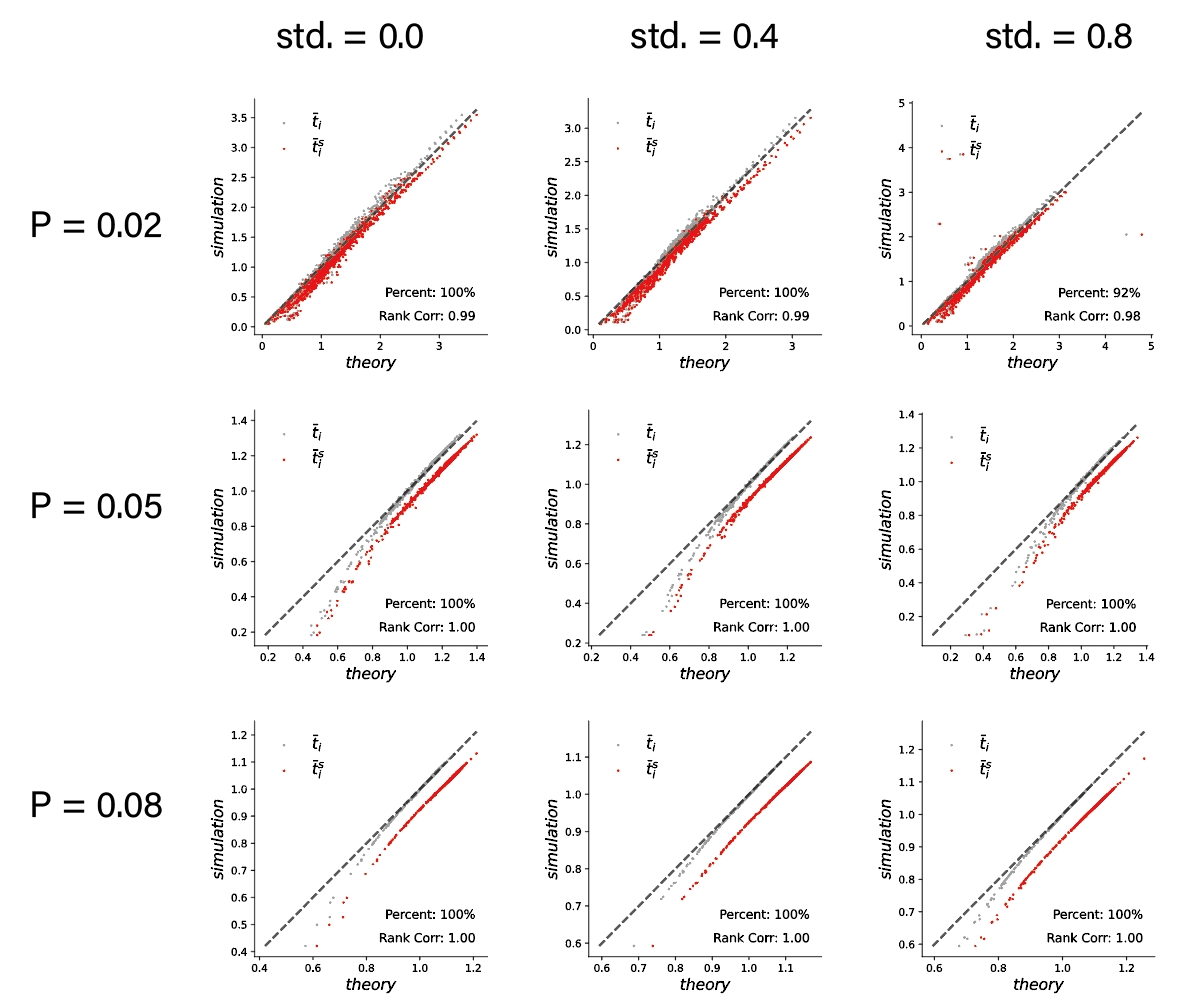}}
    \caption{Constant perturbation spreading in ER random networks ($N=100$) with Gaussian weights (mean $=10.0$, varying $std.$). Results for edge probabilities $p=0.02$ (top row), $0.05$ (middle), $0.08$ (bottom). Theoretical vs. simulated relative times ($\bar{t}_i$, $\bar{t}_i^s$) from $100$ rounds show excellent agreement, particularly with exponential estimates $\bar{t}_i$.}
\end{figure}

\begin{figure}[!ht]
    \centerline{\includegraphics[scale=0.2]{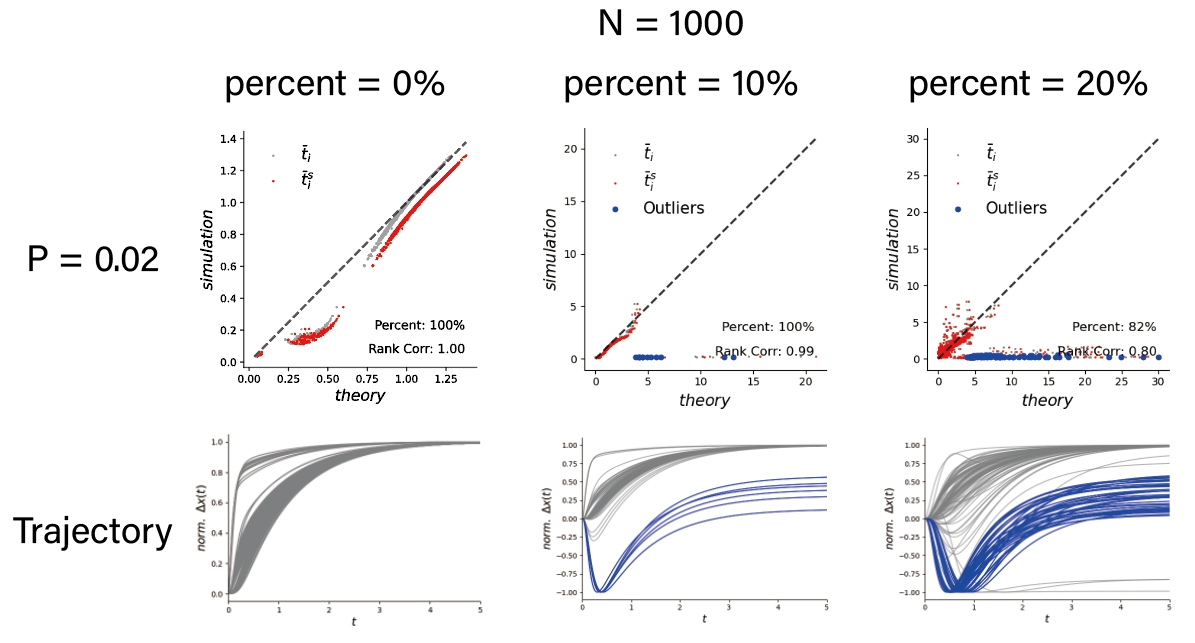}}
    \caption{Constant perturbation propagation in ER random networks with connection probability $0.02$ and varying proportions of negative links, for a network size of $1000$. Simulated and theoretical results are compared over $100$ realizations using extended relative time based on both exponential ($\bar{t}_i$) and sigmoidal ($\bar{t}_i^s$) measures. Theoretical estimates maintain high accuracy and strong rank correlations with simulation results for up to $20\%$ negative links. Beyond this threshold, increasing inhibitory links renders the system unstable.}
    \label{fig:negative:large}
\end{figure}

\begin{figure}[!ht]
    \centerline{\includegraphics[scale=0.25]{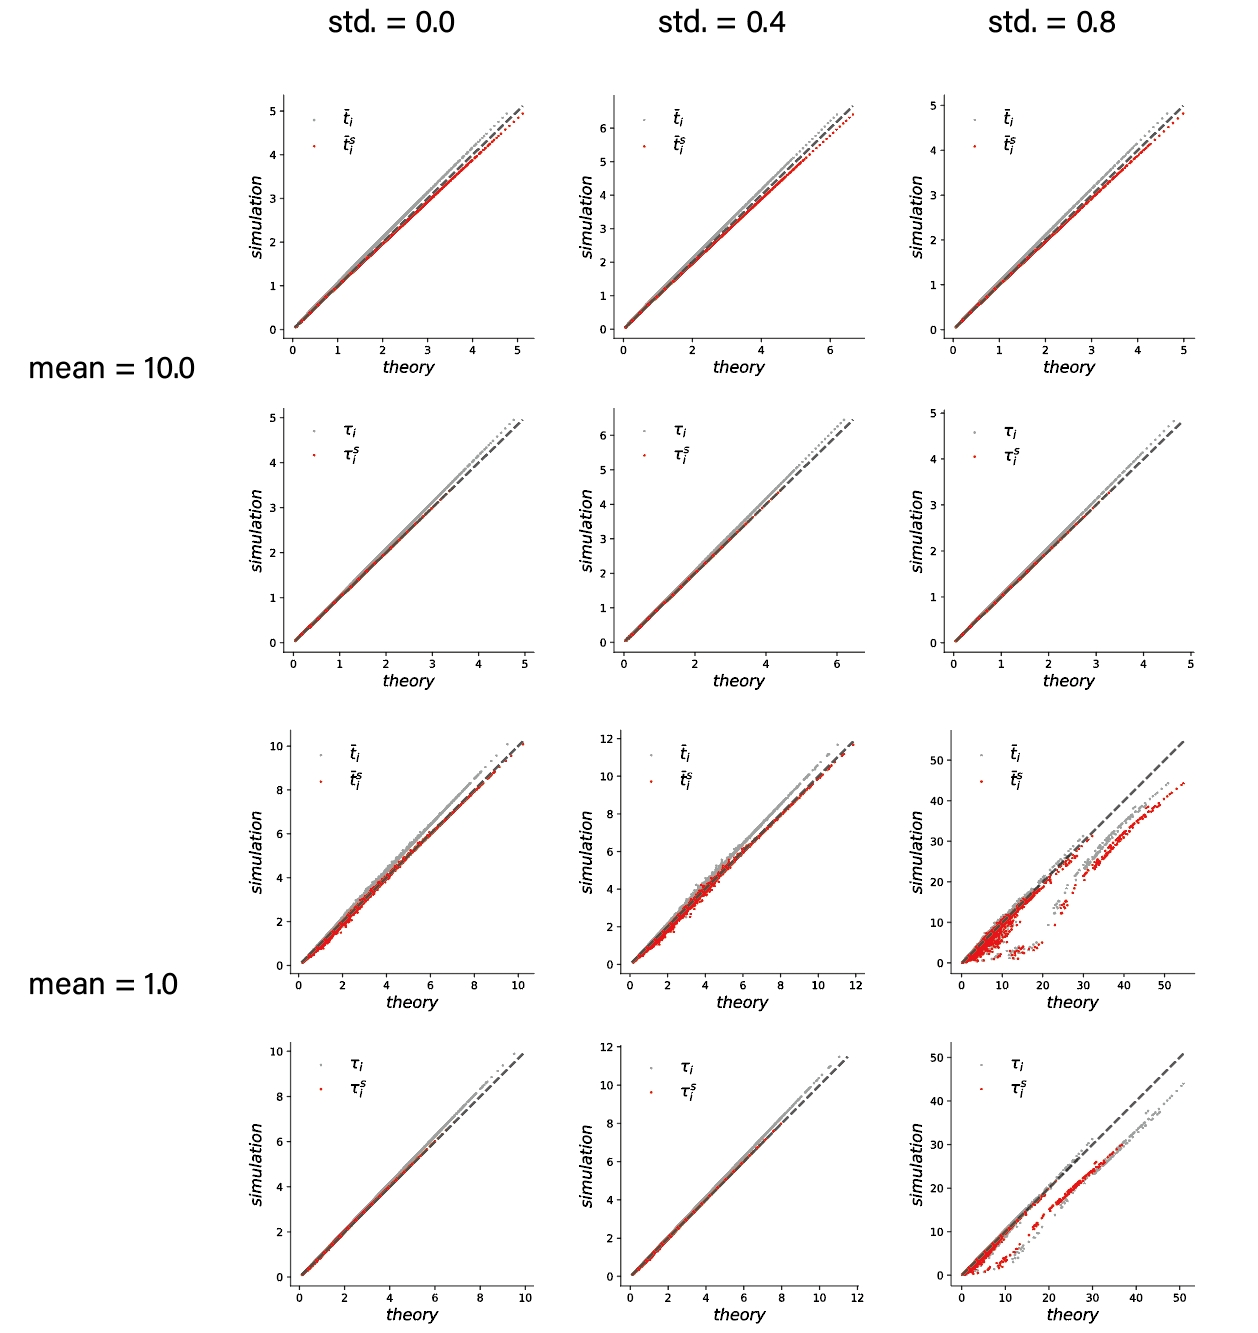}}
    \caption{Constant perturbation propagation in ER random networks with connection probability $0.02$ and network size $100$. Simulated and theoretical results for relative time are compared using both exponential ($\bar{t}_i$) and sigmoidal ($\bar{t}_i^s$) functions over $100$ realizations. The self-decay parameter is drawn from Gaussian distributions with means of $1.0$ and $10.0$, and varying standard deviations. When the mean is low, larger standard deviations reduce estimation accuracy due to the combined effects of self-decay and network interactions, causing the response traces to deviate from an exponential form, especially during the early, fast-response phase.}
\end{figure}

\begin{figure}[!ht]
    \centerline{\includegraphics[scale=0.28]{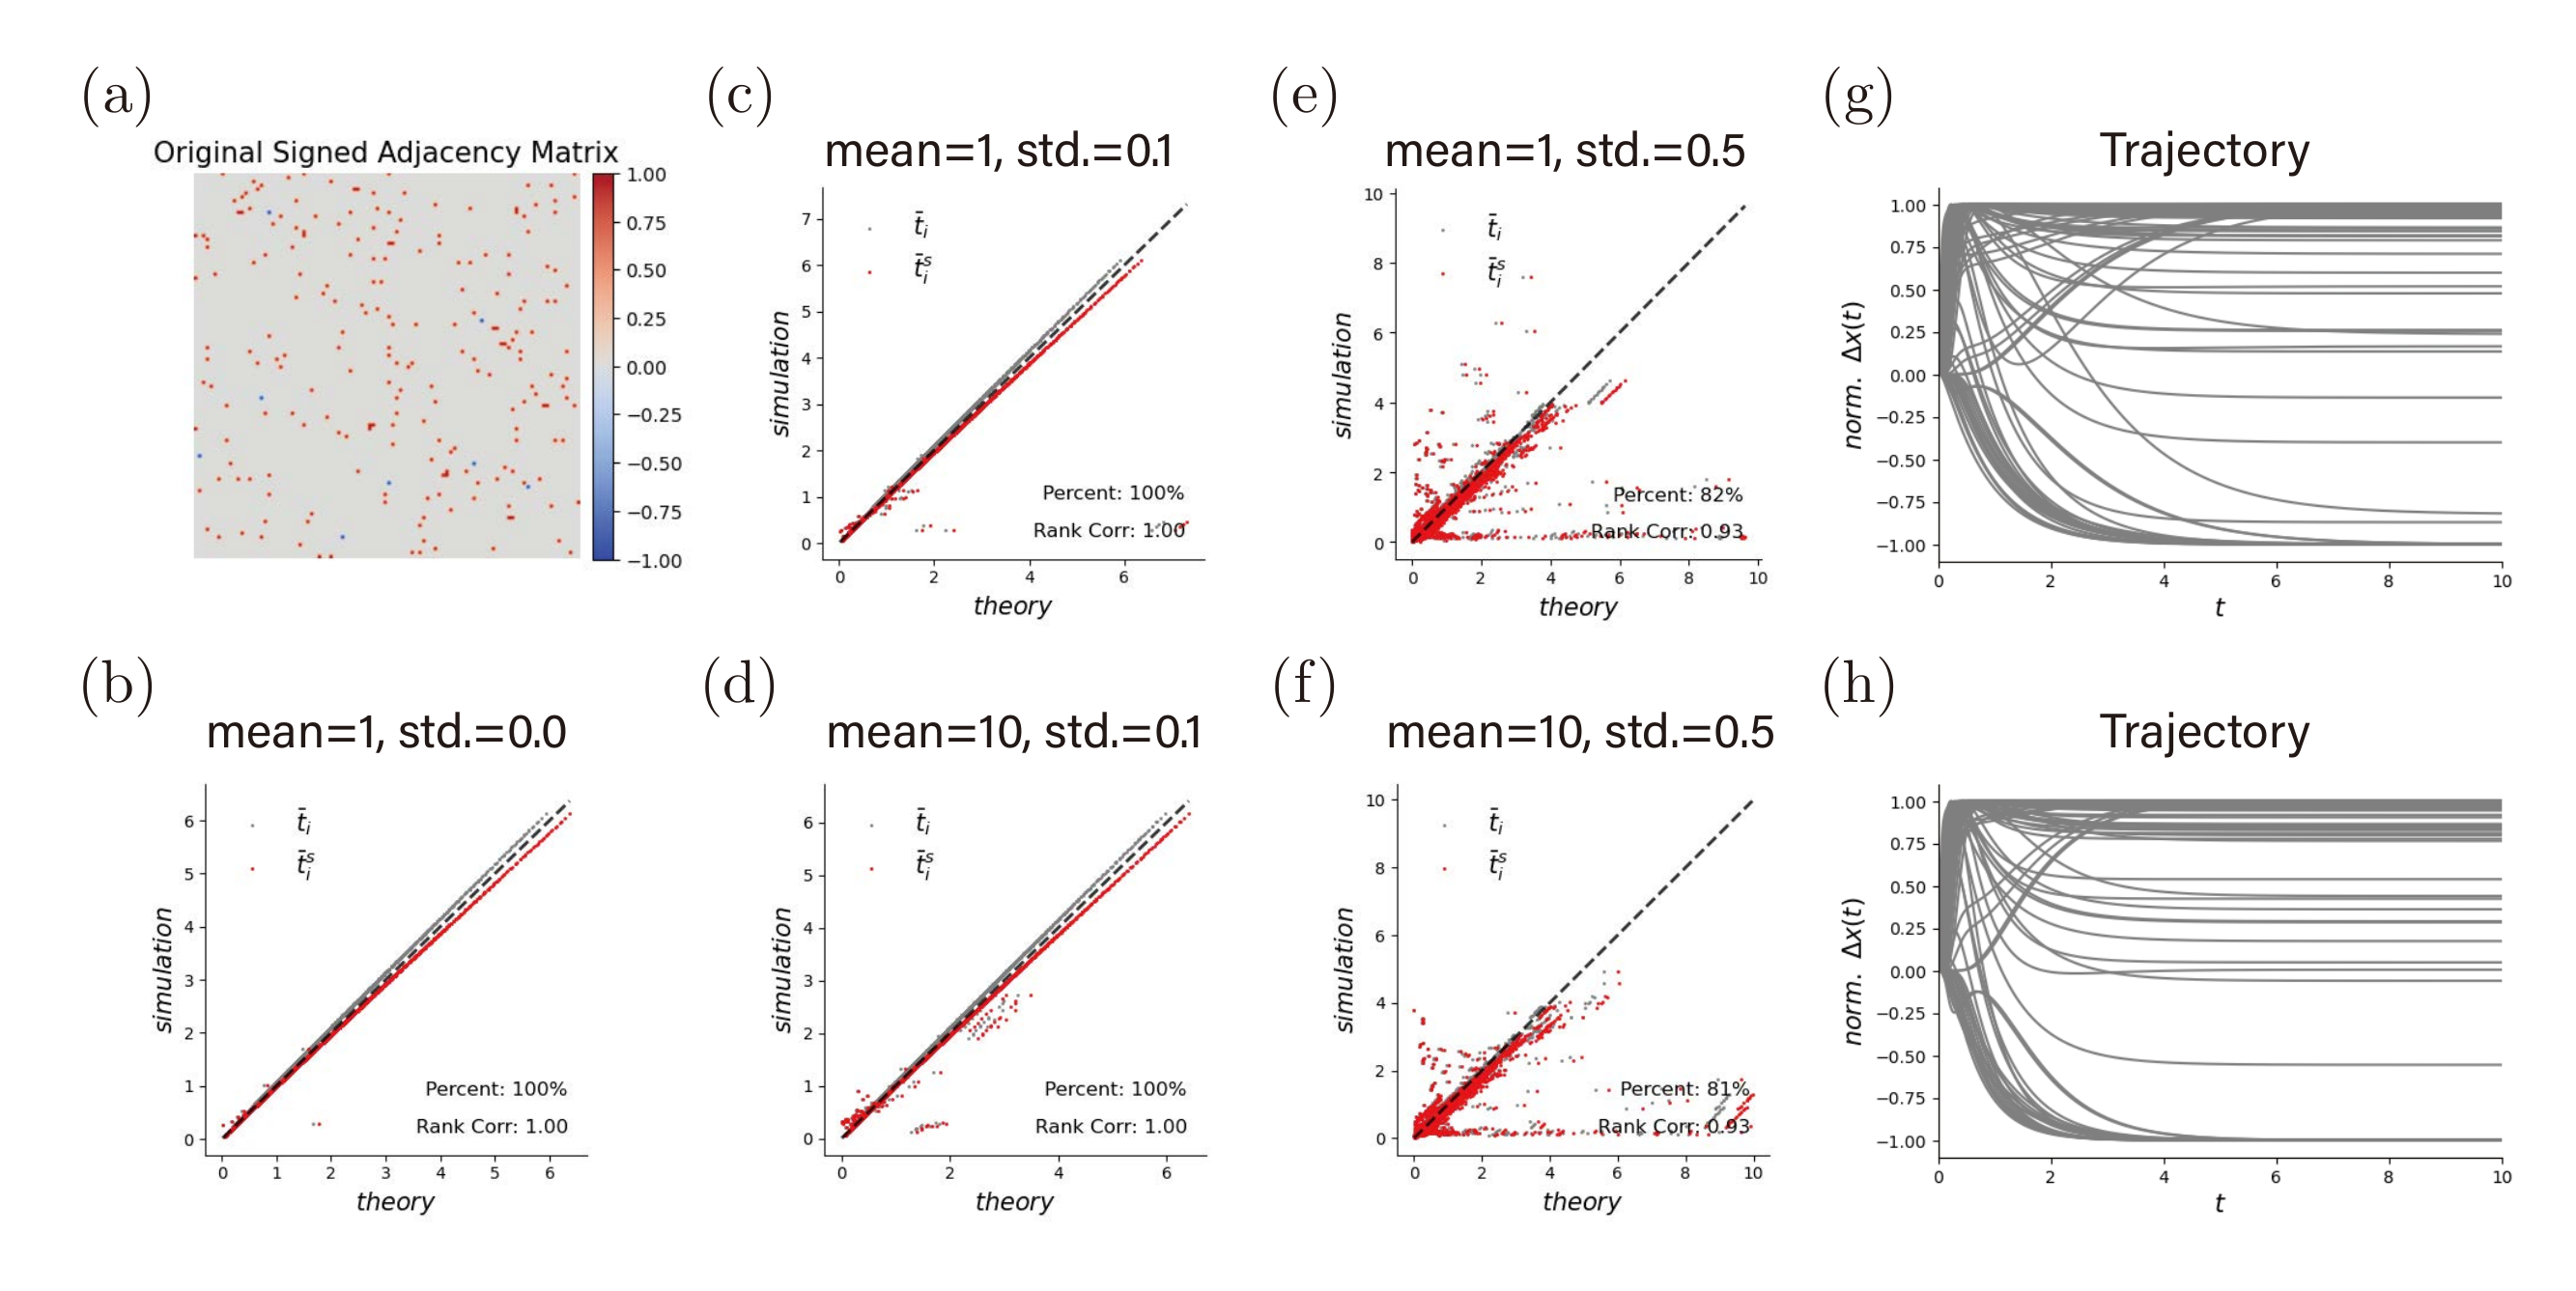}}
    \caption{Constant perturbation propagation in ER random networks with connection probability $0.02$, a fixed negative link ratio of $4\%$, and network size $100$. Simulated and theoretical results are compared for extended relative time using both exponential ($\bar{t}_i$) and sigmoidal ($\bar{t}_i^s$) functions over $100$ realizations. The self-decay parameter is set to $-11$. Increasing the standard deviation reduces accuracy, and excessively large values can lead to system instability.}
\end{figure}

\begin{figure}[!ht]
    \centerline{\includegraphics[scale=0.2]{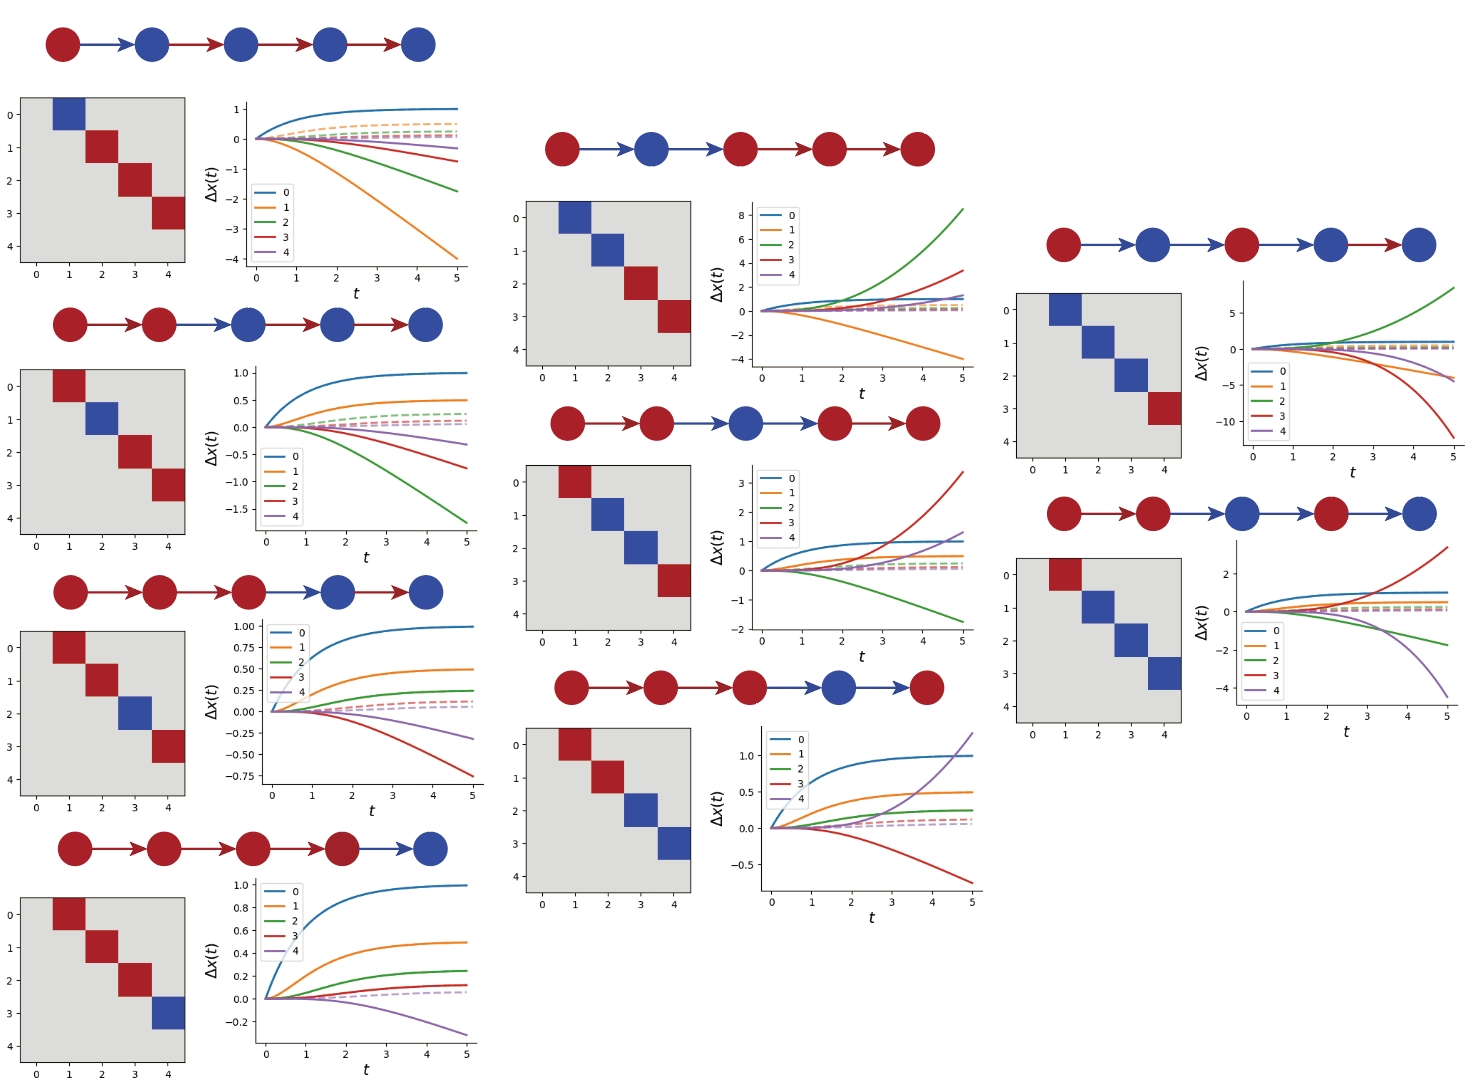}}
    \caption{Constant perturbation propagation in a directed chain with substituted negative links, indicated in blue. Node color reflects the sign of the response series, with blue denoting a sign reversal.}
\label{supp:chain:negative}
\end{figure}

\clearpage

\section{Expansion for homogeneous and heterogeneous in-degree}
\label{supp:homo}

\begin{figure}[!ht]
    \centerline{\includegraphics[scale=0.5]{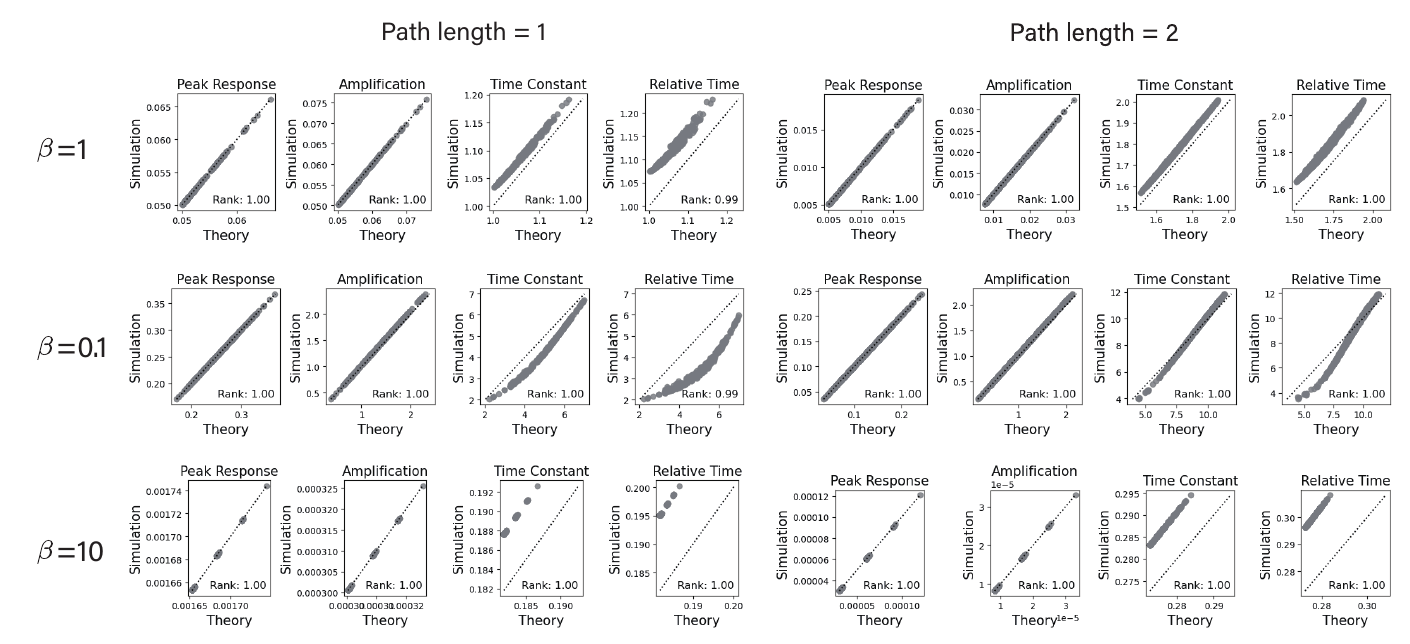}}
    \caption{Expansion under homogeneous in-degree for constant input in sparse ER random networks with varying decay rates. Theoretical expansions at order $15$ are evaluated on networks with $N = 100$ nodes and connection probability $0.05$, resulting in an average unweighted degree of $5$ and a weighted degree of $1$ (with interaction weight $\alpha = 0.2$). The response time threshold is set to $\eta = 1 - 1/e$. Although temporal estimations show a fixed numerical bias, their rank correlations remain high.}
\label{supp:homo:sparse}
\end{figure}

\begin{figure}[!ht]
    \centerline{\includegraphics[scale=0.5]{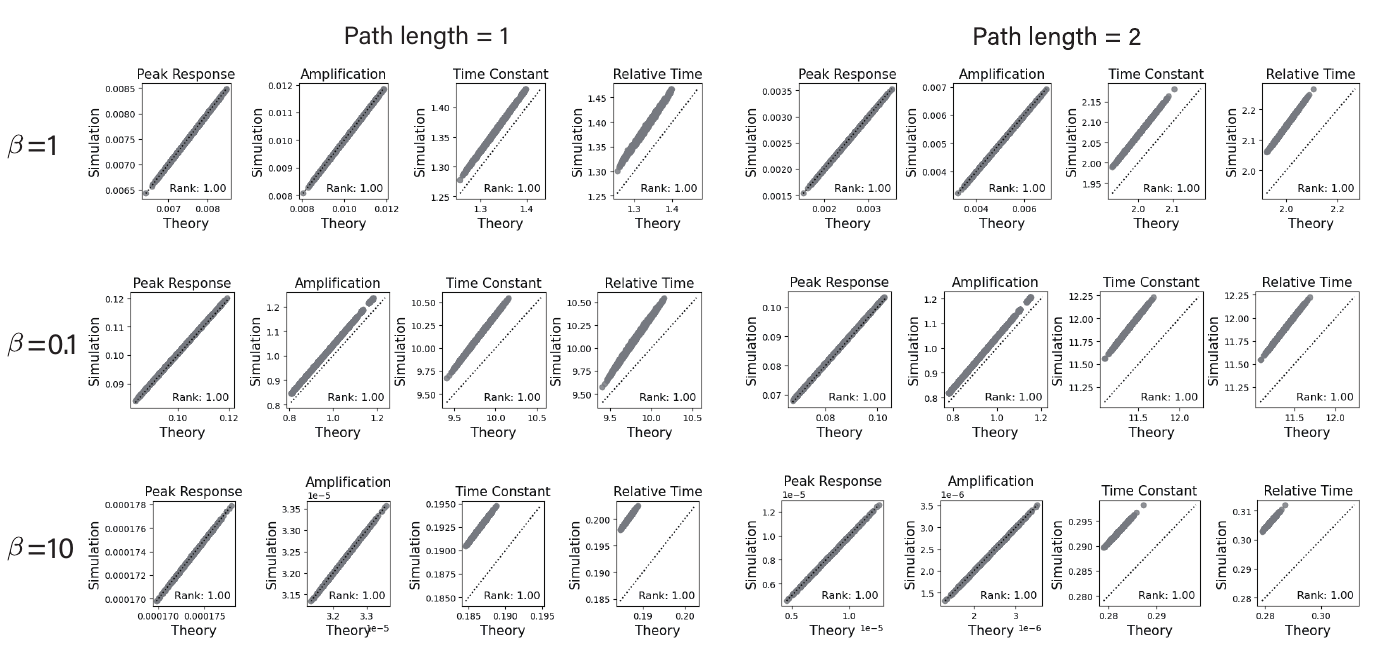}}
    \caption{Expansion under homogeneous in-degree for constant input in dense ER random networks with varying decay rates. Theoretical expansions at order $15$ are evaluated on networks with $N = 100$ nodes and connection probability $0.5$, yielding an average unweighted degree of 50 and a weighted degree of 1 (with interaction weight $\alpha = 0.02$). The response time threshold is set to $\eta = 1 - 1/e$. Although temporal estimations exhibit a fixed numerical bias, their rank correlations remain high and improve with increasing path length.}
\label{supp:homo:dense}
\end{figure}

\begin{figure}[!ht]
    \centerline{\includegraphics[scale=0.8]{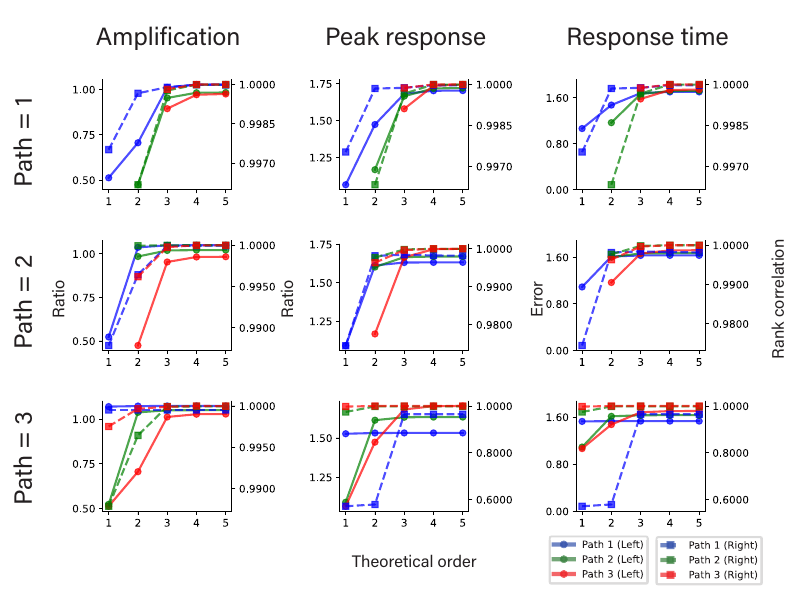}}
    \caption{Expansion accuracy for crosscovariance metrics $C_{ij}^m(\tau)$ in homogeneous in-degree ER networks with $i \neq j \neq m$. Results are averaged over $100$ realizations of networks with $N = 100$ nodes and connection probability $0.08$. The shortest path length from source node $m$ to target node $i$ is denoted as Path, while color coding—blue (Path = $1$), green (Path = $2$), red (Path = $3$)—represents the path length from $m$ to $j$. The x-axis indicates the theoretical expansion order $p$, corresponding to the power $A^p$ used in the series. For amplification, higher expansion orders and shorter paths lead to more accurate estimates and stronger rank correlations. For peak response and response time, a fixed estimation bias is present, but rank correlations still improve with increasing expansion order. Overall, deeper expansions enhance correlation performance despite persistent numerical bias.}
\label{}
\end{figure}

\begin{figure}[!ht]
    \centerline{\includegraphics[scale=0.5]{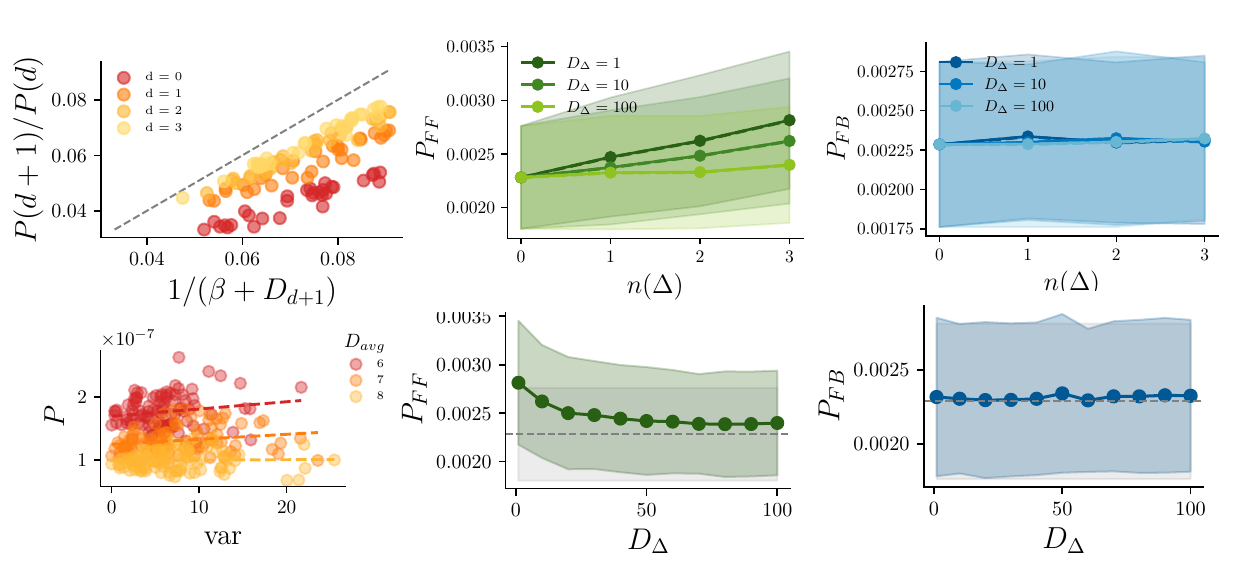}}
    \caption{Propagation of white-noise input along a single path under heterogeneous degree configurations and triangular motifs. Left (upper): A white-noise input applied to the first node $m$ produces propagation laws analogous to the constant-input case, with crosscovariance between source and target pairs scaling as ${P(d+1)}/{P(d)} \to {A_{d \to d+1}}/{(\beta + D_{d+1})}$, where $d$ is the shortest path length. Left (lower): Increasing the mean degree decreases $P$, whereas increasing degree variance enhances $P$. {Middle/Right:} Feedforward (FF) and feedback (FB) triangles amplify $P_{\mathrm{FF/FB}}$ proportionally to $n(\Delta)$, the number of triangular motifs, but with distinct slopes. Results are shown as averages over $1000$ realizations, with shading indicating $\pm 1$ SD. Large triangle-node degrees $D_\Delta$ suppress motif effects, recovering single-path dynamics ($n(\Delta)=3$). Parameters: nodal decay rate $\beta = 10$; total path length $D = 5$; input strength $I_0 = 100$; unit chain weight $A_{d \to d+1} = 1$ for all $d$.}
\label{}
\end{figure}

\begin{figure}[!ht]
    \centerline{\includegraphics[scale=0.5]{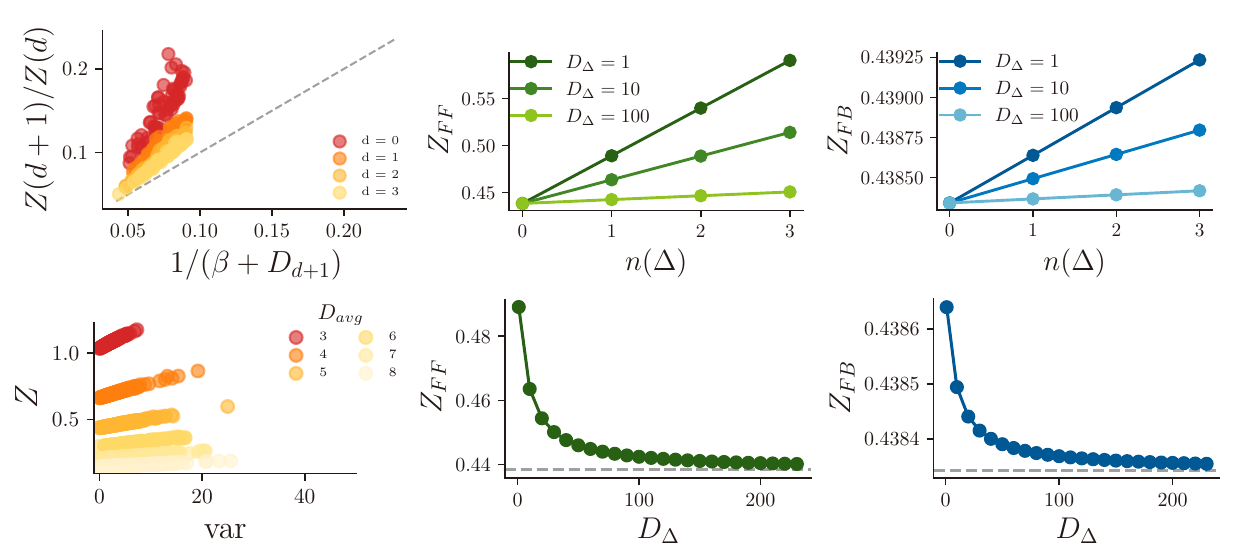}}
    \caption{Propagation of constant input along a single path under heterogeneous degree configurations and triangular motifs. Left (upper): A constant input applied to the first node $m$ produces propagation laws, with amplification between source and target pairs scaling as ${Z(d+1)}/{Z(d)} \to {A_{d \to d+1}}/{(\beta + D_{d+1})}$, where $d$ is the shortest path length. Left (lower): Increasing the mean degree decreases $Z$, whereas increasing degree variance enhances $Z$. {Middle/Right:} Feedforward (FF) and feedback (FB) triangles amplify $Z_{\mathrm{FF/FB}}$ proportionally to $n(\Delta)$, the number of triangular motifs, but with distinct slopes. Large triangle-node degrees $D_\Delta$ suppress motif effects, recovering single-path dynamics ($n(\Delta)=1$). Parameters: nodal decay rate $\beta = 10$; total path length $D = 5$; input strength $I_0 = 10^6$; unit chain weight $A_{d \to d+1} = 1$ for all $d$.}
\label{}
\end{figure}

\clearpage

\section{Numerical accuracy test for self-response}
\label{supp:self}
\begin{figure}[!h]
\centerline{\includegraphics[scale=0.5]{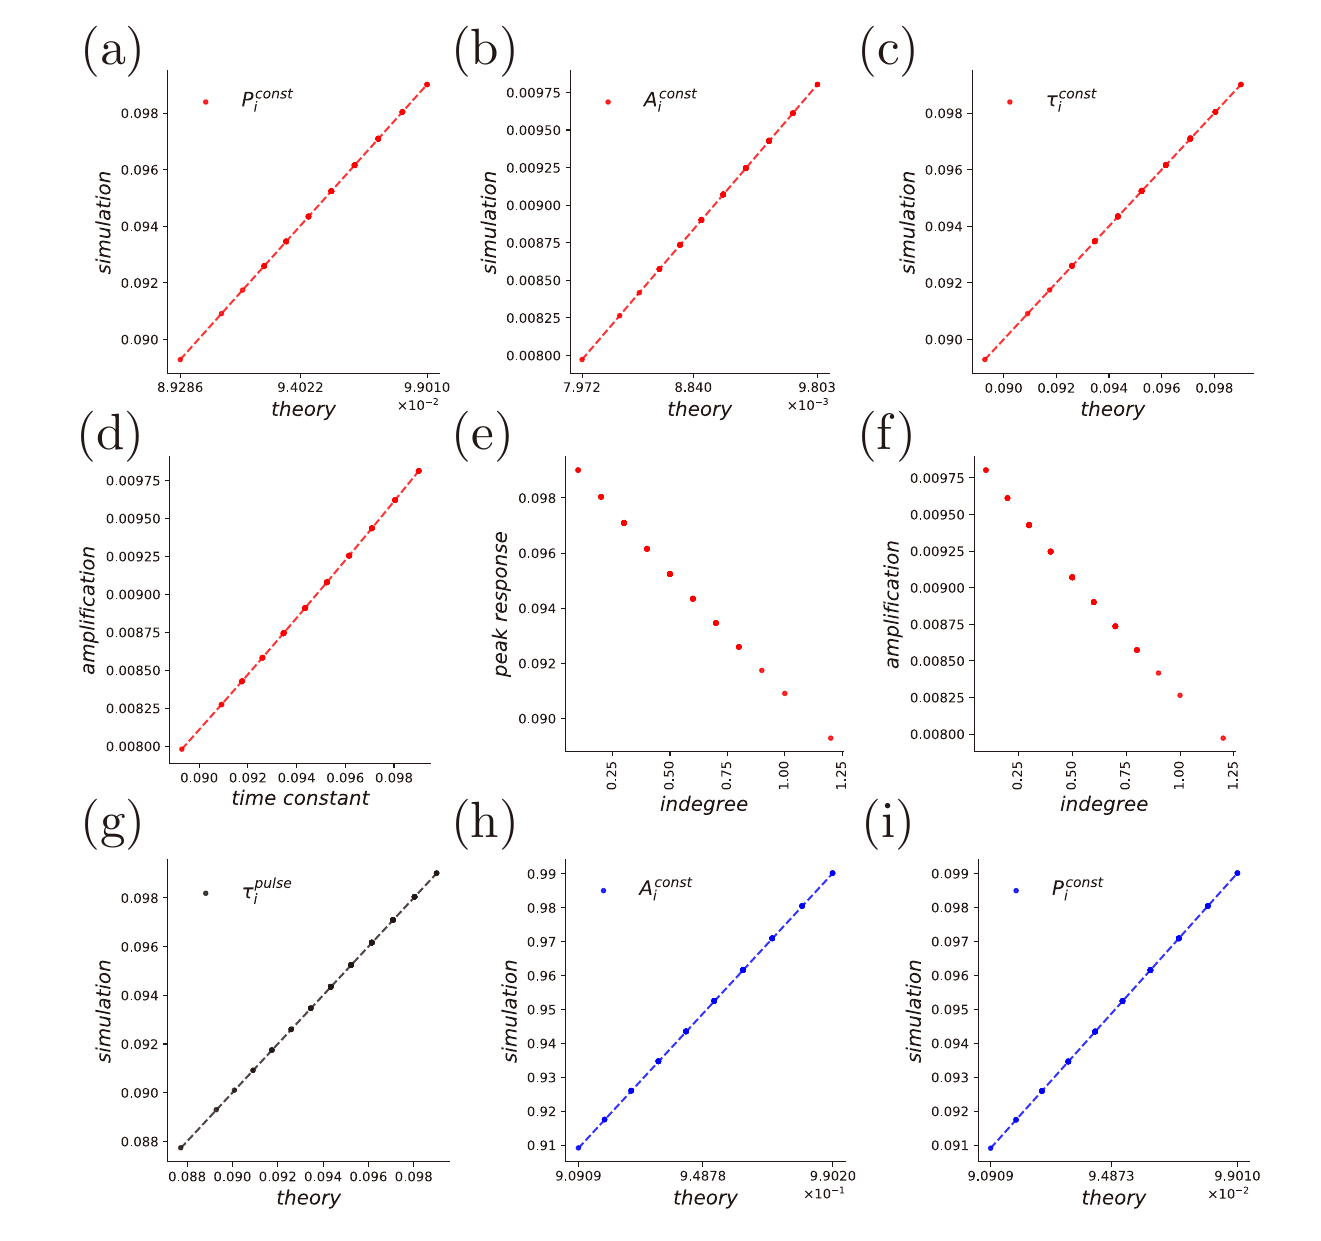}}
    \caption{Response metrics for target nodes receiving constant, pulse, and square inputs. Simulations are conducted on an ER network of size $100$, where each node receives input individually to observe its response. To satisfy expansion conditions, the interaction weight is set to $0.1$ and the self-decay parameter to $10$. (a–c) Simulated vs. theoretical results for peak response (a), amplification (b), and time constant (c) under constant input. (d) Peak response and estimated time constant share the same expression, yielding nearly identical simulated results. (e–f) Both peak response (e) and amplification (f) are inversely proportional to the indegree of the perturbed node. (g) Simulated vs. estimated time constant under pulse input. (h–i) Simulated vs. theoretical results for amplification (h) and peak response (i) under square input. Input duration is set to $10 ms$.}
\label{constant_mm}
\end{figure}

\begin{figure}[!h]
\centerline{\includegraphics[scale=0.5]{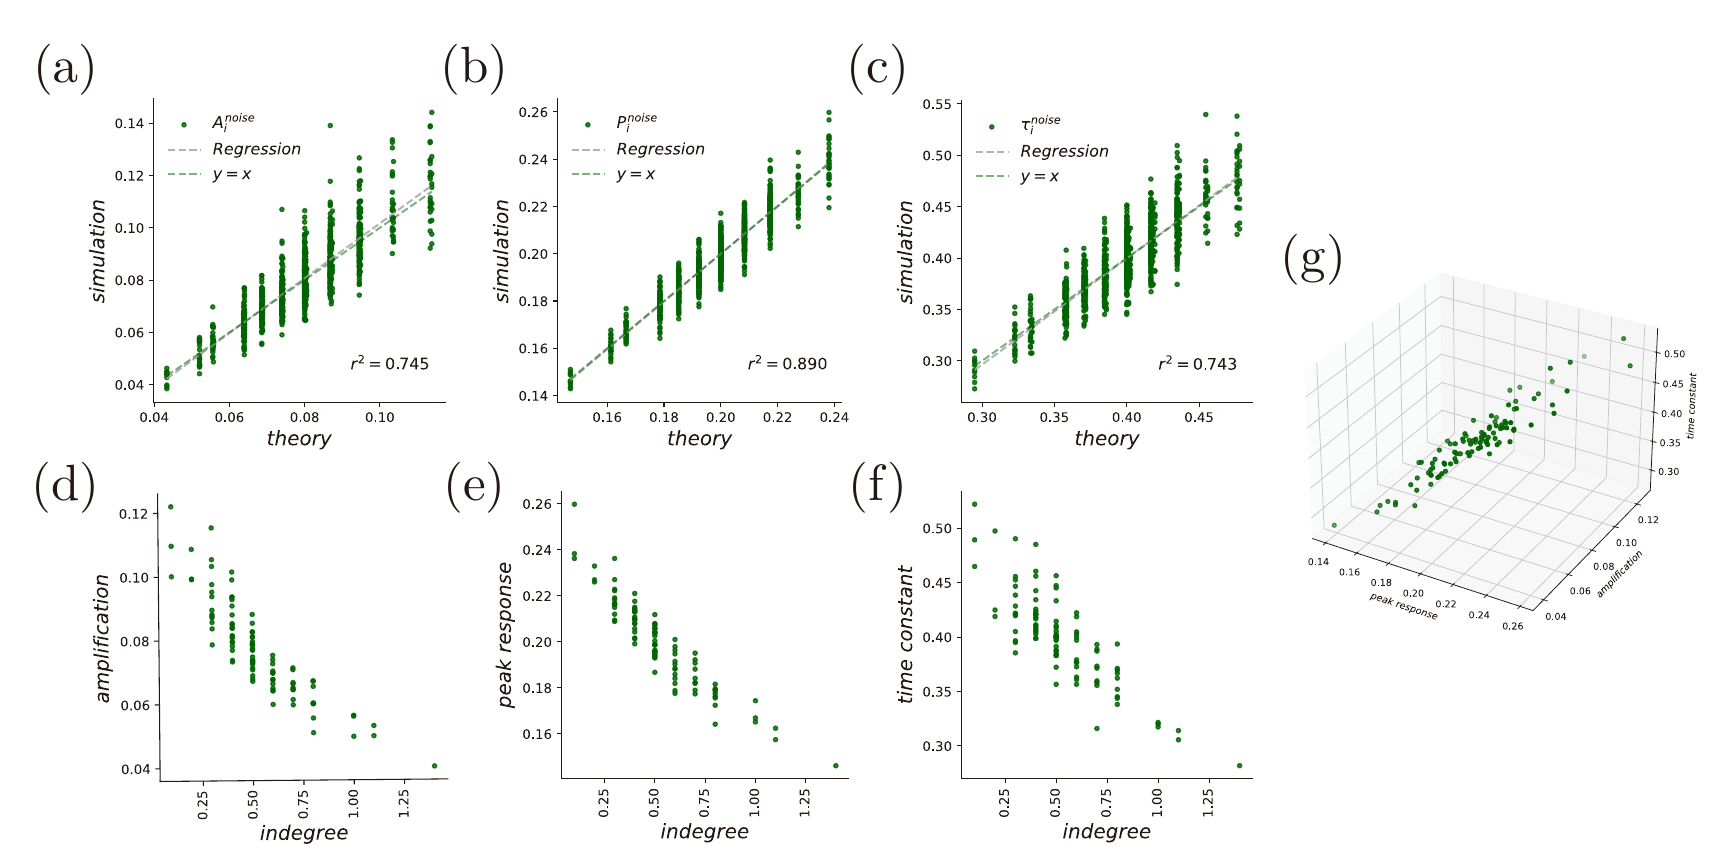}}
    \caption{
Numerical validation of theoretical estimations for self-response under noise input. Three response metrics are evaluated: amplification (a), peak response (b), and time constant (c), with theoretical predictions based on first-order truncation for simplicity. Simulations are conducted over $100$ realizations of ER random networks. All metrics show inverse dependence on nodal in-degree (d–f) and exhibit consistent trends, approximately lying along a one-dimensional manifold in the three-dimensional metric space (g).
}
\label{noise_mm}
\end{figure}

\end{document}
